# Supplementary material for: Survey of Matrix Completion Algorithms
Source: arXiv:2204.01532 source file (2022-04-05)
Supplement: Supplementary file 1 [file Supplementary.tex]

%\title{A Simple Theory for Adaptive Matrix Completion}

%\newtheorem{remark}{Remark}
%\newtheorem{lemma}{Lemma}
%\crefname{lemma}{Lemma}{Lemmas}
\newtheorem*{lemma*}{Lemma}
\newtheorem*{theorem*}{Theorem}
\newtheorem*{corollary*}{Corollary}
%\newcommand{\ilqar}[1]{{\color{red}[ilqar: #1]}}
%\newcommand{\hann}[1]{{\color{red}[hann: #1]}}
%\newcommand{\hai}[1]{{\color{red}[hai: #1]}}
%\newcommand{\ilqar}[1]{{\color{red}[ilqar: #1]}}
%\newcommand{\todo}[1]{\textcolor{red}{TODO: #1}\PackageWarning{TODO:}{#1!}}
%\renewcommand{\theenumi}{\Alph{enumi}}
%\newcommand\noisyksub{\widetilde{\mathbf{U}}^k}
%\newcommand\noisyinverse{\widetilde{\mathbf{U}}^{k^+}}
%\newcommand\projnoisy{\mathcal{P}_{\widetilde{\mathbf{U}}^k}}
%\begin{document}
%\icmltitle{A Simple Theory for Adaptive Matrix Completion}
\maketitle

\section{Proof of the Lemma \ref{lm1}, Exact Recovery with Sparsity Number}

We start with rephrasing the lemma 1 and provide further discussions regarding \textit{space sparsity}.
Later, we are using the idea of the lemma and design an algorithm that has similar flavor to \hyperlink{ks2013}{$\mathbf{KS2013}$} with the difference that this method recovers the underlying matrix deterministically.

\subsection{Proof of lemma \ref{lm1}}

\begin{lemma*}\label{lem:zero-num-lin-dependence} Let $\mathbb{U}$ be a subspace of $\mathbb{R}^{m}$ and $x^1,x^2,...,x^n$ be any set of vectors from $\mathbb{U}$. Then the linear 
dependence of $x^1_\Omega, x^2_\Omega,..., x^n_\Omega$ implies linear dependence of 
$x^1,x^2,...,x^n$ for any $\Omega \subset [m]$ such that $|\Omega| > \overline{\psi}(\mathbb{U})$.
\end{lemma*}

\begin{proof}%[\bf Proof ]  
By the hypothesis of linear dependence, there are coefficients 
$\alpha_1, ... , \alpha_{n}$, not all 
zero, such that 
\begin{align*}
\alpha_1 x^1_\Omega + ... + \alpha_{n} x^n_\Omega = 0.     
\end{align*}
To show linear dependence of $x^1,\ldots, x^n$ we prove the following equation also satisfies
\begin{align*}
\alpha_1 {x^1} + ... + \alpha_{n} {x^n}=0     
\end{align*}
Assume by contradiction 
$y= \sum_{i=1}^{k} \alpha_i {x_i}$
is a nonzero vector.  But, we have
\begin{align*}
y_\Omega= \sum_{i=1}^{k} \alpha_i {x_i}_\Omega =0    
\end{align*}
which implies $\overline{\psi}(\mathbb{U}) \geq |\Omega|$ from the definition of \textit{space sparsity number}. 
However, $|\Omega| > \overline{\psi}(\mathbb{U})$ from the hypothesis of the lemma which concludes a contradiction.
Therefore, the assumption the vector $y$ being nonzero vector cannot be true, then the following satisfies : 
\begin{align*}
 y= \sum_{i=1}^{k} \alpha_i {x_i} = 0   
\end{align*}
\end{proof}
\hspace{-6mm}In the following lemma we prove somewhat reverse statement of the lemma 1. 
\begin{lemma}\label{lem:zero-num-lin-dependence} Let $\mathbb{U}$ be a subspace of $\mathbb{R}^{m}$ and $x^1,x^2,...,x^n$ be any set of vectors from $\mathbb{U}$. Then the linear 
dependence of ${x^1}, {x^2},...,{x^n}$ implies linear dependence of 
$x^1_\Omega, x^2_\Omega,...,x^n_\Omega$, for any $\Omega \subset [m]$.
\end{lemma}
\begin{proof}%[\bf Proof ]  
The proof of the statement is straightforward observation of the fact that 
$$\alpha_1 {x^1} + ... + \alpha_{n} {x^n}=0 $$
implies 
$$\alpha_1 x^1_\Omega + ... + \alpha_{n} x^n_\Omega = 0_\Omega = 0 $$    
\end{proof}
\textbf{Tightness of lemma 1:}
We show example for tightness of the lemma with the following matrix:
\[ \mathbf{M} = \begin{bmatrix}
    1       & 2 & 5 \\
    1       & 2 & 4 \\
    1       & 0 & 4 \\
    1       & 0 & 4
\end{bmatrix} \]
First observation here is columns of $\mathbf{M}$ is linearly independent.
Then, the next observation is that $e_1 = (1,0,0,0)$ is contained in the column space.
Therefore, the \textit{space sparsity number} of the column space of $\mathbf{M}$ is at least equal to $3$.
Using the fact that \textit{space sparsity number} is less then 4 we conclude that column \textit{space sparsity number} is exactly equal to $3$.
Lets check the submatirx $\textbf{M}_{\Omega:}$ where $\Omega=\{2,3,4\}$: 
\[ \mathbf{M_{\Omega:}} = \begin{bmatrix}
    1       & 2 & 4 \\
    1       & 0 & 4 \\
    1       & 0 & 4
\end{bmatrix} \]
Columns of $\mathbf{M_{\Omega:}}$ is linearly dependent (first and third column), however columns of $\mathbf{M}$ is not. 
Then, it follows that there is an example that when $\| \Omega \| =\overline{\psi}(\mathbb{U}) $ but the hypothesis of the lemma 1 not satisfied.
Therefore, the statement of the lemma 1 is tight.

\begin{lemma} \label{lem:bds}
For the column space $\mathbb{U}$ of $m\times n$ sized matrix $\mathbf{M}$ with rank-$r$, the following inequality is satisfied $$r-1 \leq \overline{\psi}(\mathbb{U}) \leq m-1.$$ 
\end{lemma}
\begin{proof}
$\overline{\psi}(\mathbb{U}) < m $ is straightforward because any  nonzero vector in $\mathbb{R}^{m}$ has at most $m-1$ coordinates equal to zero.
Then, it follows from the definition of the \textit{space sparsity number}, $\overline{\psi}(\mathbb{U}) \leq m-1$. \medskip \\
In the rest of the proof we prove $r-1 \leq \overline{\psi}(\mathbf{M})$.
$\mathbf{M}$ having rank $r$ implies that we can choose $r$ rows from it that are the basis for the row space of it. 
Technically, we may find $R\subset [m]$ such that $|R| = r$ and $\mathbf{M}_{R:}$ is rank $r$. 
Similarly, we can find $C\subset [n]$ such that $|C| = r$ and $\mathbf{M}_{R:C}$ is an $r \times r$-sized matrix of rank $r$. 
It follows that there exists $\alpha \in \mathbb{R}^r$ such that $$\mathbf{M}_{R:C} \alpha = e_1 = \big(1,0,\ldots,0\big).$$ 
Consequently, $\mathbf{M}_{:C}\alpha \neq 0$ but has zero components in $r-1$ of the indices given by $R$. 
Thus $\overline{\psi}(\mathbf{M}_{:C} )\geq r-1$. 
Finally: $$ r-1 \leq \overline{\psi}(\mathbf{M}_{:C} ) \leq \overline{\psi}(\mathbb{U})$$
\end{proof}
\paragraph{Discussion for lemma \ref{lem:bds}:} It is easy to construct examples to show both sides of the inequality  is tight (i.e. equality satisfied).
For any matrix that $e_1=\big(1,0,0,\ldots,0\big)$ is contained in the column space, $\overline{\psi}(\mathbb{U})=m-1$ is trivially correct.\medskip \\
Moreover, column space of the general rank-$r$ matrices creasted as $\mathbf{M}= \mathbf{X} \mathbf{Y}$ where $\mathbf{X}\in \mathbb{R}^{m\times r} $ and $\mathbf{X}_{i,j} \sim \mathcal{N}(0,1)$, $\mathbf{Y}\in \mathbb{R}^{r\times n}$ and $\mathbf{Y}_{i,j} \sim \mathcal{N}(0,1)$ left side of the inequality is tight (i.e. $r-1=\overline{\psi}(\mathbb{U})$).\medskip \\
\subsection{Exact Recovery with Sparsity Number}
The algorithm below-$\mathbf{ERCS}$ is just modification of the algorithm $\hyperlink{ks2013}{\mathbf{KS2013}}$ in the input phase. 
We show observing just $d=\overline{\psi}(\mathbb{U})+1$ many entries in each column is enough te decide whether partially observed column is contained in the subspace or not.\medskip\\
Under the condition that the column space $\mathbb{U}$ of the underlying matrix satisfies $r-1=\overline{\psi}(\mathbb{U})$, the observation complexity of the algorithm $\mathbf{ERCS}$ becomes $m\times r +(n-r)\times r = (m+n-r) r$ which is the degree of freedom of the set of $m\times n$ sized rank-$r$ matrices.
Therefore, under this condition $\mathbf{ERCS}$ is absolutely optimal
%\ilqar{performing in optimal rate sometimes. degree of freedom and stuff.}

\begin{algorithm}
\caption*{ \hypertarget{ercs}{\textbf{ERCS: }}Exact recovery with column sparsity}
 \textbf{Input:}   $d=\overline{\psi}(\mathbb{U})+1$

 \textbf{Initialize:}  $k=0 , \widehat{\mathbf{U}}^0 = \emptyset$ 

\begin{algorithmic}[1]
    \STATE Draw uniformly random entries $\Omega \subset [m]$ of size $d$   
    \STATE Observe entire $\mathbf{M}_{\Omega:}$ 
    \FOR{$i$ from $1$ to $n$}        
    \STATE  \hspace{0.2in} \textbf{if} $\| \mathbf{M}_{\Omega:i}-\mathcal{P_U}_{\Omega} \mathbf{M}_{\Omega:i}\| >0$ 
    \STATE \hspace{0.2in}  \hspace{0.2in} Fully observe $\mathbf{M}_{:i}$ 
    \STATE  \hspace{0.2in}  \hspace{0.2in}  $\widehat{\mathbf{U}}^{k+1} \leftarrow \widehat{\mathbf{U}}^{k} \cup \mathbf{M_{:i}} $
    \STATE \hspace{0.2in}  \hspace{0.2in} Orthogonalize  $\widehat{\mathbf{U}}^{k+1}$
    \STATE \hspace{0.2in} \hspace{0.2in} $k=k+1$          
   \STATE   \hspace{0.2in}  \textbf{otherwise:} $\widehat{\mathbf{M}}_{:i} = \widehat{\mathbf{U}}^k \widehat{\mathbf{U}}^{k^+}_{\Omega:} \widehat{\mathbf{M}}_{\Omega :i}$
\ENDFOR

\end{algorithmic}
 \textbf{Output:} Underlying matrix $\widehat{\mathbf{M}}$
\end{algorithm}

\begin{theorem}
Let $\mathbb{U}$ represent the column space of the $m\times n$  sized matrix $\mathbf{M}$ of rank $r$. 
Then, $\hyperlink{ercs}{\mathbf{ERCS}}$ exactly recovers $\mathbf{M}$ by $$m\times r  + (n-r)(\overline{\psi}(\mathbb{U})+1)$$
observations.
\end{theorem}
\begin{proof}%[\bf Proof]  
We start by showing $\mathbf{ERCS}$ recovers $\mathbf{M}$ exactly and later we focus on observation count.
To prove correctness of exact recovery we use mathematical induction as follow:\medskip \\
$Hypothesis$ : after $i$-th iteration $\mathbf{ERCS}$ already  correctly recovered first $i$ columns. \medskip \\
$Base$ $case$ : $i=1$ is trivial as if at least one of the observed entries is nonzero we completely observe the column, which guarantees correctness. 
On the other hand, if it happens all of $\overline{\psi}(\mathbb{U})+1$ entries are zero, then the first column is indeed completely zero because the definition of the \textit{space sparsity number} implies there can be at most $\psi(\mathbb{U})$ many zero coordinates in a nonzero vector in the column space.\medskip\\
$Hypothesis$ $proof$ : 
Let assume after step $i-1$, $\mathbf{ERCS}$ recovered first $i-1$ columns correctly and we want to show the algorithm exactly recovers $i$-th column too.\medskip\\
From the design of the algorithm $\mathbf{M}_{\Omega : {i}}$ is already observed.
Then, if in the line 4, $\mathbf{ERCS}$ decides the column is linearly independent with previous columns, as in the next line we completely observe the column there is no chance that the algorithm can do mistake under this case.
Therefore, the only remaining case is, if in the line 4 the algorithm decides the column $i$ is linearly dependent.\medskip\\
From the statement of lemma 1, if a set of vectors from a subspace $\mathbb{U}$ are linearly dependent on a given subset of coordinates, then they are indeed linearly dependent. 
We conclude that the algorithm's decision is correct and by just back projection method, the algorithm recovers remaining entries of the partially observed column.
Therefore, column $i$ also recovered correctly and we are done with the proof of induction hypothesis. \medskip\\
Our next goal is to show the observation complexity is $m\times r  + (n-r)(\overline{\psi}(\mathbb{U})+1)$.
From the lemma 1, we conclude that whenever current column is indeed linearly independent with previous columns, the $\mathbf{ERCS}$ also decides it is linearly independent.
Moreover, from the lemma 10, we conclude that if the current column is linearly dependent with previous columns, then in this case $\mathbf{ERCS}$ decides it is linearly dependent.
As there are $r$ many linearly independent columns in the underlying matrix $\mathbf{M}$, the algorithm decides independence exactly $r$ times and in each of them it does complete observations.
However, in remaining $n-r$ columns, number of observations is exactly $\overline{\psi}(\mathbb{U})+1$.
As a conclusion, number of total observations is: $rm+(n-r)(\overline{\psi}(\mathbb{U})+1)$
\end{proof}
\begin{corollary}
$\mathbf{ERCS}$ still performs correctly under the case in each column, number of observed entries is lower bounded by $\overline{\psi}(\mathbb{U})$ : $d \geq \overline{\psi}(\mathbb{U})+1$. Moreover, the number of observations will be $m\times r + (n-r)d$ 
\end{corollary}
\begin{proof}%[\bf Proof] 
The proof is exactly proceeds as proof of the theorem.
The key point is to notice, lemma 1 and lemma 10 are still satisfying.
\end{proof}
\paragraph{Optimality of $\mathbf{ERCS}$:}
We notice that both of algorithms $\hyperlink{ks2013}{\mathbf{KS2013}}$ and $\hyperlink{ercs}{\mathbf{ERCS}}$ has two stages of observation.
\begin{itemize}
    \item[$i:$] Select subset of rows and observe them completely.
    \vspace{-3mm}
    \item[$ii:$] Detect linearly independent columns and observe them completely.
\end{itemize}
The discussion for tightness of the lemma 1 above implies that $\mathbf{ERCS}$ is optimal deterministic two stage observation, low-rank exact recovery algorithm.
Moreover, in the corollary above we discussed for any $d\geq \overline{\psi}(\mathbb{U})$ 
the $\mathbf{ERCS}$ algorithm would still perform correctly.
Therefore, having constant factor approximation of the \textit{space sparsity number} of the column space would lead asymptotically optimal algorithm:
\begin{align*}
  \widehat{d} \leq K d & \implies \widehat{d}+1 \leq K(d+1)     \\
  & \implies   (n-r)(\widehat{d}+1) \leq (n-r)K(d+1)            
\end{align*}
adding $mr$ to both side leads to
\begin{align*}
      rm+ (n-r)(\widehat{d}+1) &\leq rm +(n-r)K(d+1)            \\
                               & \leq Krm + K(n-r)(d+1)         \\
                               & = K\big(rm+(n-r)(d+1)\big)
\end{align*}
Notice that $rm+ (n-r)(\widehat{d}+1)$ is the observation complexity we have and $\big(rm+(n-r)(d+1)\big)$ is optimal two stage as we discussed here.
All together, the inequality above implies constanct approximation to \textit{space sparsity number} gives as constant approximation to optimal solution.

\section{Exact Recovery with Heterogeneous Cost}

Here, we discuss matrix completion problem with relatively different setting.
Previously, we focused on the case, where each of the entry of underlying matrix $\mathbf{M}$ has the same observation cost.
In this section we discuss the completion problem where entries of the matrix has non uniform cost to observe.
We tackle with two type of non uniformity here: 
\begin{itemize}
    \item Entries has uniform cost across the same column, but different columns has different costs. 
    \item Each entry of the matrix has different cost.
\end{itemize}
\subsection{Uniform Cost Across Columns}

\textbf{Problem:} For any fixed $j$, the cost of observing $\mathbf{M}_{i:j}$ is equal to $\chi_j$ for any $1\leq i \leq m$, and $\chi_1, \chi_2,\ldots, \chi_n$ are arbitrary positive numbers and we target to recover the matrix $\mathbf{M}$ as cheap as possible. \medskip\\
\textbf{Solution:} We propose a slight modification of the \hyperlink{ercs}{$\mathbf{ERCS}$} to solve optimally among the two staged methods as we discussed before.
Lets remind that in the algorithm we show that selecting any $d=\overline{\psi}(\mathbb{U})+1$ many rows is enough to guarantee exact recovery deterministically.
In the next stage, we iteratively go through columns one by one starting with the first column, and if we detect a column is linearly independent with previous ones, we completely observe it.
If not, we recover it using the pre-determined subspace.\medskip\\
To adapt the solution for this problem, we just need to change the order of the columns we start to check. 
Basically, instead of starting with the first column, we should start with the cheapest one.
If we decide its not contained in the current subspace, we completely observe all entries and if it is contained then we just recover with the current subspace.
Then, we move to second cheapest column and so on so forth with the increasing order of cost.\medskip\\
%\begin{algorithm}
%\caption*{\textbf{ERCSUCC: }Exact recovery with column space sparsity under condition of uniform observation cost within each column}
% \textbf{Input:}  $d$ \\
% \textbf{Initialize:} $\widehat{\mathbf{M}}$ set to $m\times n$ sized null matrix, $\widehat{\mathbb{U}}^0=\emptyset$, $k=0$
%\begin{algorithmic}[1]\label{algj}
%    \STATE Select any set of $d$ columns $\Omega \subset [m]$    
%    \STATE Measure entire $\mathbf{M}_{\Omega:}$ 
%    \STATE $i_1,i_2,...,i_n$ is permutation of $1,2,...,n$ such that  $c_{i_1}, c_{i_2}, ... ,c_{i_n}$ is non-decreasing 
%    \FOR{j from 1 to n}        
%    \STATE  \hspace{0.2in} \textbf{if} $\| \mathbf{M}_{\Omega:{i_j}}-\mathcal{P_U}_{\Omega} \mathbf{M}_{\Omega:{i_j}}\| >0$ 
%    \STATE \hspace{0.2in}  \hspace{0.2in} Fully Measure $\mathbf{M}_{:{i_j}}$ 
%    \STATE  \hspace{0.2in}  \hspace{0.2in}  $\widehat{\mathbf{U}}^{k+1} \leftarrow \widehat{\mathbf{U}}^{k} \cup \mathbf{M_{:{i_j}}} $
%    \STATE \hspace{0.2in}  \hspace{0.2in} Orthogonalize  $\widehat{\mathbf{U}}^{k+1}$
%    \STATE \hspace{0.2in} \hspace{0.2in} $k=k+1$          
%   \STATE   \hspace{0.2in}  \textbf{otherwise:} $\widehat{\mathbf{M}}_{:i} = \widehat{\mathbf{U}}^k \widehat{\mathbf{U}}^k_{\Omega} \widehat{\mathbf{M}}_{\Omega :{i_j}}$
%\ENDFOR
%\STATE return $\widehat{\mathbf{M}}$ 
%\end{algorithmic}
% \textbf{Output:} Underlying matrix $\widehat{\mathbf{M}}$
%\end{algorithm}
\textit{Correctness:} We can see that the proof of the correctness of $\mathbf{ERCS}$ is independent of the order of the columns. 
Therefore, selecting columns with increasing order of the cost would not change the correctness of the algorithm. \medskip\\
\textit{Optimality:} The set of two stage algorithm can be parametrized by two numbers. 
First one is - $d$- the number of rows fully observed and the second is the subset of indices of columns to observe fully. 
We analyse the optimal algorithm for three cases of values of $d$:\\\\
1. $d \leq \overline{\psi}(\mathbb{U})$. 
It is obvious that optimal algorithm cannot have $d \leq \overline{\psi}(\mathbb{U})$, because from the discussion for tightness of the lemma \ref{lm1} and optimality of $\mathbf{ERCS}$, there are matrices that selection of $d = \overline{\psi}(\mathbb{U})$ rows is not enough to guarantee the existence of $r$ linearly independent rows.
\medskip\\
2. $d = \overline{\psi}(\mathbb{U})+1$ It is a well known fact that the set of column basises are matroids and Greedy algorithms gives the optimal solution for matroids \cite{matroid}.
Note that the algorithm designed above is efficient way of giving greedy solution.
\medskip\\
3. $d > \overline{\psi}(\mathbb{U})+1$. Lets assume that the optimal algorithm takes $\Tilde{d}>d$ rows in the first phases and  columns: $i_1,i_2,\ldots, i_{\Tilde{r}}$. 
We first note that, $\Tilde{r}=r$, it is because if $\Tilde{r}<r$ then selected columns are not enough to learn the column space and if $\Tilde{r}>r$  we can pick subset of these columns that is basis for column space and selecting this basis has less cost which contradicts to optimality. Therefore, $\Tilde{r}=r$ for optimal case.
Moreover, we can use the same subset selection argument to pick $\overline{\psi}(\mathbb{U})+1$ sized subset of rows then select the same set of columns and it will be cheaper.
Therefore, for optimality we should select exactly $d= \overline{\psi}(\mathbb{U})+1$ rows.

\subsection{Exact recovery with full heterogeneity }
\textbf{Problem:} For any $i,j$, the cost of observing $\mathbf{M}_{i:j}$ is equal to $\chi_{ij}$ and $\chi_{11}, \chi_{12},\ldots, \chi_{mn}$ are arbitrary positive numbers and similar to the previous problem we target to recover the matrix $\mathbf{M}$ as cheap as possible. \medskip\\
\textbf{Solution:} We describe the solution in the following algorithm:
\begin{algorithm}
\caption*{\textbf{ERHC: } \hypertarget{erhc}{Exact} recovery with heterogeneous cost}
 \textbf{Input:}  $d = \overline{\psi}(\mathbb{U})+1$ here $\mathbb{U}$ is the column space of the underlying matrix \\
 \textbf{Initialize:} $\widehat{\mathbf{M}}$ set to $m\times n$ sized null matrix, $\widehat{\mathbf{U}}^0=\emptyset$, $k=0$

\begin{algorithmic}[1]\label{algj}
    \FOR{$i$ from $1$ to $m$,}
    \STATE $\chi^i =\sum_{j=1}^{n}\chi_{ij}$ 
    \ENDFOR
    
    \STATE Sort $\chi^i$s with increasing order and select first $d$ and denote their index set by$-R$         
    \STATE Observe entire $\mathbf{M}_{R:}$ 
    \FOR{$i$ from $1$ to $m$,}
    \STATE $\overline{\chi}^i =\sum_{j\in[n]\setminus R}\chi_{ij}$ 
    \ENDFOR

    \STATE Sort $\overline{\chi}^i$s with increasing order and lets denote $\{i_1,i_2,\ldots,i_n\}$ as $\overline{\chi}^{i_1} \leq \overline{\chi}^{i_2} \leq \ldots \leq  \overline{\chi}^{i_n}$

    \FOR{$h$ from $1$ to $m$,}
    \STATE \hspace{0.2in} \textbf{If} $\| \mathbf{M}_{R:i_h}-\mathcal{P}_{\widehat{\mathbf{U}}^k_{R}} \mathbf{M}_{R :i_h}\|^2 >0$ 
    \STATE \hspace{0.4in} Fully observe $\mathbf{M}_{:i_h}$ add it to the basis                 $\widehat{\mathbf{U}}^k$
    \STATE \hspace{0.4in} Orthogonalize  $\widehat{\mathbf{U}}^k$
    \STATE \hspace{0.4in} $k=k+1$ 
    \STATE \hspace{0.2in} \textbf{Otherwise:} $\widehat{\mathbf{M}}_{:i_h} = \widehat{\mathbf{U}}^k \widehat{\mathbf{U}}^{k^+}_{R:} \widehat{\mathbf{M}}_{R : i_h}$
\ENDFOR

    \STATE return $\widehat{\mathbf{M}}$ 

\end{algorithmic}
 \textbf{Output:} Underlying matrix $\widehat{\mathbf{M}}$
\end{algorithm}

\paragraph{Correctness:} We can see the correctness of $\mathbf{ERHC}$ is due to the correctness of $\mathbf{ERCS}$ as selecting cheapest $\overline{\psi}(\mathbb{U})+1$ is special case of selecting any $\overline{\psi}(\mathbb{U})+1$ many columns and iteration order over the columns doesn't matter similarly for this case too.

\paragraph{Optimality:} Unlike to the previous case, greedy algorithm doesn't give us the cheapest combination of columns and rows. 
Following example provides a matrix and entry costs that shows that greedy algorithm is not optimal.
\[ 
\mathbf{M} = \begin{bmatrix}
    1       & 1 & 2 & 3\\
    1       & 2 & 3 & 4\\
    1       & 3 & 4 & 5\\
    1       & 4 & 5 & 6
\end{bmatrix} 
\hspace{10mm}\mathbf{\chi} = \begin{bmatrix}
    1   & 1 & 4 & 1 \\
    1   & 5 & 3 & 4\\
    4   & 3 & 4 & 4\\
    1   & 4 & 4 & 8
\end{bmatrix} 
\]
The greedy algorithm for this case observes rows $R=\{1,2\}$  and columns $C= \{1,2\}$ which has overall cost of:
\begin{align*}
 (1+1+4+1)+(1+5 &+3+4) +(4+1) +(3+4)   = 32
\end{align*}
However, observing ${R}=\{1,3\}$  and columns ${C}= \{1,3\}$ would give us overall cost of:
\begin{align*}
 (1+1+4+1)+(4+3 +4+4) +(1+1) +(3+4) = 31
\end{align*}
which is cheaper than greedy algorithm.\\\\
However, with the same cost matrix, there are other matrices that shares the same column space as $\mathbf{M}$ (therefore the same column space sparsity number) but greedy algorithm is still optimal.
For the same cost matrix with a slightly modified underlying matrix, we can give an example:
\[ 
\overline{\mathbf{M}} = \begin{bmatrix}
    1       & 1 & 2 & 2\\
    1       & 2 & 2 & 3\\
    1       & 3 & 2 & 4\\
    1       & 4 & 2 & 5
\end{bmatrix} 
\hspace{10mm}\mathbf{\chi} = \begin{bmatrix}
    1   & 1 & 4 & 1 \\
    1   & 5 & 3 & 4\\
    4   & 3 & 4 & 4\\
    1   & 4 & 4 & 8
\end{bmatrix} 
\]
This gives us the conclusion, with just information of the observation cost matrix and column space sparsity number, we cannot pick theoretical optimal set of rows and columns that is guaranteed carrying all of information of the underlying matrix.
\paragraph{2-Optimality:} Even though greedy algorithm cannot return the optimal set of rows and columns, here we show that the overall cost of the cost oof the algorithm is at most twice expensive than optimal. \medskip\\
We denote the row set and column set parameter of optimal 2-stage algorithm $\tilde{R}$ and $\tilde{C}$ and cost of it by $\sigma_{OPT}$.
Then, we can decompose optimal soluton into its parts as following:
    $$\sigma_{OPT}=\chi(\mathbf{M}_{\tilde{R}:}) + \chi(\mathbf{M}_{:\tilde{C}}) - \chi    (\mathbf{M}_{\tilde{R}:\tilde{C}})$$.
Trivially,  both of the following inequalities satisfied 
$$\chi(\mathbf{M}_{\tilde{R}:\tilde{C}}) \leq  \chi(\mathbf{M}_{:\tilde{C}})$$
$$\chi(\mathbf{M}_{\tilde{R}:\tilde{C}}) \leq  \chi(\mathbf{M}_{\tilde{R}:})$$
which these inequalities implies that  $$\sigma_{OPT} \geq \mathrm{max}(\chi(\mathbf{M}_{:\tilde{C}}) , \chi(\mathbf{M}_{\tilde{R}:})).$$
Now lets decompose cost of greedy algorithm to its pieces:
    $$\sigma_{G}=\chi(\mathbf{M}_{R:}) + \chi(\mathbf{M}_{:C}) - \chi(\mathbf{M}_{R:C})$$
Note that the greedy algorithm doesn't necessarily selects cheapest basis columns, however selected columns minimizes the overall cost after rows selected. 
Therefore, we conclude that if we denote the set of cheapest columns by $C^B$, then the following inequality satisfied:\\\\
\begin{align*}
\sigma_{G} =\chi(\mathbf{M}_{R:}) + \chi(\mathbf{M}_{:C}) - \chi(\mathbf{M}_{R:C})     
& \leq \chi(\mathbf{M}_{R:}) + \chi(\mathbf{M}_{:C^B}) - \chi(\mathbf{M}_{R:C^C})  \\[1.2ex]
& \leq 2 \hspace{1mm} \mathrm{max}\big(\chi(\mathbf{M}_{R:}) , \chi(\mathbf{M}_{:C^B}) \big)
\end{align*}
As we discussed before in order to have guarantee that we will be able to have full information to detect linearly independent columns we need to observe at least $\psi(\mathbb{U})+1$ many rows.\medskip\\
Moreover, as greedy algorithm observe exactly $\overline{\psi}({\mathbb{U}})+1$ many rows by choosing cheapest columns we are guaranteed to have:
$$ \chi(\mathbf{M}_{R:}) \leq  \chi(\mathbf{M}_{\tilde{R}:})$$
Similarly as $C^B$ represents the set of cheapest columns, we have:
$$ \chi(\mathbf{M}_{:C^B}) \leq  \chi(\mathbf{M}_{:\tilde{C}})$$
which together implies 
$$ \mathrm{max}\big(\chi(\mathbf{M}_{R:}), \chi(\mathbf{M}_{:C^B}) \big) \leq  \mathrm{max}\big(\chi(\mathbf{M}_{\tilde{R}:}), \chi(\mathbf{M}_{:\tilde{C}}) \big).$$
Putting all inequalities together we conclude:
\begin{align*}
\sigma_G \leq 2 \hspace{1mm}\mathrm{max}\big(\chi(\mathbf{M}_{R:}) , \chi(\mathbf{M}_{:C^B}) \big)
\leq 2 \hspace{1mm} \mathrm{max}\big(\chi(\mathbf{M}_{\tilde{R}:}) , \chi(\mathbf{M}_{:\tilde{C}}) \big) 
\leq 2 \sigma_{OPT}
\end{align*}
Therefore, we conclude that greedy algorithm gives us 2-optimal algorithm.\\
\paragraph{Tightness:} In the following example, we see that greedy algorithm cannot guarantee better than 2-optimality:\\
\[ \mathbf{\chi} = \begin{bmatrix}
    \frac{\epsilon}{100}   & \frac{\epsilon}{100} & \frac{\epsilon}{100} & \frac{\epsilon}{100} & 10-\epsilon & 10-\epsilon  \medskip\\
    \frac{\epsilon}{100}   & \frac{\epsilon}{100} & \frac{\epsilon}{100} & \frac{\epsilon}{100} & 10-\epsilon & 10-\epsilon  \medskip\\
    10  & 10 & \frac{\epsilon}{100} & \frac{\epsilon}{100} & \frac{\epsilon}{100} & \frac{\epsilon}{100}  \medskip \\
    10  & 10 & \frac{\epsilon}{100} & \frac{\epsilon}{100} & \frac{\epsilon}{100} & \frac{\epsilon}{100} \medskip \\
    \frac{\epsilon}{100}  & \frac{\epsilon}{100} & 10 & 10 & 10-\epsilon & 10-\epsilon \medskip\\
    \frac{\epsilon}{100}  & \frac{\epsilon}{100} & 10 & 10 & 10-\epsilon & 10-\epsilon \medskip\\
\end{bmatrix} 
\]\medskip\\
It is clear that optimal choice is ${C}=\{1,2\}$ and ${R}=\{3,4\}$ which gives the cost of :
$$\sigma_{OPT} = 10+10+10+10 + 16 \times \frac{\epsilon}{100} =40 + \frac{\epsilon}{6.25}$$
However, greedy algortihm will pick ${R}=\{1,2\}$ in the first stage which has overall cost of 
$$(10-\epsilon)+(10-\epsilon)+(10-\epsilon)+(10-\epsilon) + 8 \times \frac{\epsilon}{100} =40-4\epsilon+   \frac{\epsilon}{12.5}$$
Then in the next stage it choose columns ${C}=\{5,6\}$ which also has cost of 
$$(10-\epsilon)+(10-\epsilon)+(10-\epsilon)+(10-\epsilon) + 4 \times \frac{\epsilon}{100} =40-4\epsilon + \frac{\epsilon}{25}$$
 which all together cumulative cost is 
 $$(40-4\epsilon) +   \frac{\epsilon}{12.5} + (40-4\epsilon) +   \frac{\epsilon}{25}= 80-8\epsilon + \frac{3}{25}\epsilon.$$
 To find the fraction of this cost to optimal cost we get
 $$\frac{\sigma_G}{\sigma_{OPT}} = \frac{80-8\epsilon + \frac{2\epsilon}{25}}{40+\frac{\epsilon}{6.25}}  \approx 2 -\frac{\epsilon}{5}.$$
Therefore for any number smaller than $2$, we can choose an $\epsilon$ which ratio of the cost of greedy algorithm to optimal set is larger than that number.
This implies that, 2-optimality of the algorithm \hyperlink{erhc}{$\mathbf{ERHC}$} is tight.
\newpage

\section{Proof of Theorem \ref{thm:lg2}. Exact Recovery for Low Rank Matrices. }

We start with rephrasing the theorem 2 and then divide the theorem into two parts and prove them separately.
\begin{theorem*}(Exact Recovery for Low-Rank Matrices)  
Let $r$ be the rank of underlying $m\times n$ sized matrix $\mathbf{M}$ with column space $\mathbb{U}$ and row space $\mathbb{V}$. 
Then,  \hyperlink{err}{$\mathbf{ERR}$} exactly recovers the underlying matrix $\mathbf{M}$ with probability at least $1-\epsilon$  using at most 
$$(m+n-r)r +  \mathrm{min}\Big(  2 \frac{m n}{{\psi}(\mathbb{U})}\log{(\frac{r}{\epsilon})} , \frac{\frac{2m}{\psi(\mathbb{U})}(r+2 +\log{\frac{1}{\epsilon}})}{\psi(\mathbb{V})}n \Big)  $$
observations.
\end{theorem*}
We split the statement of the theorem above into two and prove each of them separately.
First, we show that observation complexity is upper bounded by $(m+n-r)r +  2 \frac{m n}{{\psi}(\mathbb{U})}\log{(\frac{r}{\epsilon})} $.
Then, in another theorem we show that the observation complexity is bounded by 
$$(m+n-r)r + \frac{\frac{2m}{\psi(\mathbb{U})}(r+2 +\log{\frac{1}{\epsilon}})}{\psi(\mathbb{V})}  $$
and the statement of theorem follows from these two results.

\subsection{Matrices with Incoherent Row Space}

\begin{theorem*}[ Highly coherent row space] 
Let $r$ be the rank of underlying $m\times n$ sized matrix $\mathbf{M}$ with column space $\mathbb{U}$. 
Then,  $\mathbf{ERR}$ exactly recovers the underlying matrix $\mathbf{M}$ with probability at least $1-\epsilon$  using at most 
$$(m+n-r)r +  2 \frac{m n}{{\psi}(\mathbb{U})}\log{(\frac{r}{\epsilon})}  $$
observations.
\end{theorem*}

\begin{proof}%[\bf Proof]
The proof is consisting following steps: 
\begin{itemize}
\item \textit{step 1.} Give terminology will be used throughout the proof. Identifying type of observations to two classes : informative and  non-informative.
\item \textit{step 2.} Provide a bound to number of informative observations.
\item \textit{step 3.} In remaining steps, we try to give bound to non-informative observations. We start by giving upper bound to the unsuccessful observations in line 5.
\item \textit{step 4.} We model the execution of  $\mathbf{ERR}$ with a stochastic process and design another process which terminates faster than this.
\item \textit{step 5.} We relate the problem to basic combinatorial counting  problem and analyse
\item \textit{step 6.} Conclude that total number of observations is 
\begin{align*}
(m+n-r)r +  2 \frac{m n}{{\psi}(\mathbb{U})}\log{(\frac{r}{\epsilon})}.
\end{align*}

\end{itemize}
\textit{Step 1:}
For ease of readability we denote $\psi(\mathbb{U})$ by $k$ during the proof.
Lets start a process in the beginning of the algorithm for each column. 
We call process of the column $\mathbf{M}_{:j}$ dies in one of the following cases happens:
\begin{itemize}
    \item[a.] $\mathbf{M}_{:j}$ is fully observed in line 6 in some intermediate step of  $\mathbf{ERR}$
    \item[b.] $\mathbf{M}_{:j}$ is contained in the column space of the already fully observed columns in underlying matrix $\mathbf{M}$ (i.e. columns in $C$).
    \item[c.]  Algorithm already learns entire column space : $\widehat{r} = r $
\end{itemize}
If a column/process is not dead then we call it is active.
We call an observation is informative if it is observed at line 6 (i.e. it contributes to the studied column/row space learned by  $\mathbf{ERR}$ and uninformative if it observed at line 3. 
Obviously some entries are observed both at line 3 and 6, so they count in both non-informative and informative observations. \\\\
\textit{Step 2:}
We can simply observe that the number of informative observations is exactly $m r + n r - r^2$. 
Because, at the end of the algorithm set of informative observations is just set of $r$ many linearly independent columns (we have $mr$ observations here) and $r$ many linearly independent rows (we have $nr$ observations here). 
By observing that entries in $r\times r$ sub-matrix is counted twice, we conclude that overall observations is just 
\begin{align*}
  mr + nr - r^2   
\end{align*}
\textit{Step 3:} In order to give upper bound to the number of non-informative observations, we see it is enough to bound the number of phases the algorithm  $\mathbf{ERR}$ passes through.
Specifically, if the number of phases is bounded by $T$ then overall number of non-informative observations is bounded by $Tn_2$. 
In order to give upper bound to $T$, we first explore the probability of an detecting independence of an observation in line 3 for an active column:
\begin{lemma} \label{lemma:prob_bound}
The probability of detecting independence of an active column in the $j$'th phase of the algorithm  $\mathbf{ERR}$ is lower bounded by $\frac{k}{m-j}$
\end{lemma}
\begin{proof}
In an intermediate step of  $\mathbf{ERR}$ we have $|C| = |R| = \widehat{r}$ and   $M_{R:C}$ is $\widehat{r} \times \widehat{r}$ matrix of rank $\widehat{r}$. 
Then, for any $i\in [n]$, $\mathbf{M}_{R:i}$ is in the column space of $\mathbf{M}_{R:C}$ as the matrix is full rank and therefore its column space is entire $\mathbb{R}^{\widehat{r}}$. 
Then there exists unique coefficients $\alpha_1, \alpha_2, ...,\alpha_{\widehat{r}}$
for columns $C =\{c_1,...,c_{\widehat{r}}\}$ that following equality satisfied.
\begin{align*}\alpha_1 \mathbf{M}_{R:c_1} + \ldots + \alpha_{\widehat{r}} \mathbf{M}_{R:c_{\widehat{r}}}  = \mathbf{M}_{R:i} 
\hspace{5mm}\implies \hspace{5mm} \alpha_1 \mathbf{M}_{R:c_1} + \ldots + \alpha_{\widehat{r}} \mathbf{M}_{R:c_{\widehat{r}}}  - \mathbf{M}_{R:i} = 0
\end{align*}
Now, let observe the vector 
\begin{align*} 
y=\alpha_1 \mathbf{M}_{:c_1} + \alpha_2 \mathbf{M}_{:c_2}  + ... + \alpha_{\widehat{r}} \mathbf{M}_{:c_{\widehat{r}}}  - \mathbf{M}_{:i} 
\end{align*} 
We know that $y\neq 0$ because we know 
column $i$ is linearly independent with previous observed columns -
$\mathbf{M}_{:c_1}, \mathbf{M}_{:c_2},..., \mathbf{M}_{:c_{\widehat{r}}}$.
Moreover for any row index $a\in R$,  $y_a =0$ because $y_R =0$
from the definition of $\alpha_j$'s. 
As $y$ is in the column space of $M$ it has at most $m-k$-many zero coordinates. 
Moreover, for any $a \notin R$ but $\mathbf{M}_{i_a:i}$ observed in line 6 
$y_{i_a}=0$ should satisfy, because otherwise in one of previous iterations we 
would already decide $\mathbf{M}_{:i}$ is linearly independent and we would add index $i$ to $C$, but here we know $i\notin C$. \medskip\\
Basically we conclude that all known coordinates of $y$ is 0 and number of 
known coordinates is represented by $observed$.
We know at least $k$  many coordinates of $y$ is nonzero and we already have $m-observed$ many coordinates of $y$ is zero, then with probability at least: $\frac{k}{m-observed}$ uniformly selected next observation will be zero.
Being nonzero of $y_a$ implies non-singularity of the matrix $\mathbf{\widehat{M}}_{\widehat{R}:\widehat{C}}$ where 
$\widehat{R}=R\cup\{a\}$ and $\widehat{C}=C\cup \{i\}$. It is because if this matrix was not 
invertible then there would 
be coefficients $\beta_1,...,\beta_{r'+1}$ (not all of them are zero) such that 
\begin{align*}
\beta_1 \mathbf{M}_{\widehat{R}:c_1} + ... + \beta_{\widehat{r}} \mathbf{M}_{\widehat{R}:c_{\widehat{r}}} + \beta_{\widehat{r}+1} \mathbf{M}_{\widehat{R} : i}  = 0.    
\end{align*} 
From lemma 2, linear independence of $\mathbf{M}_{R:c_1}, \mathbf{M}_{R:c_{\widehat{r}}} $ implies linear independence of $\mathbf{M}_{\widehat{R}:c_1}, \mathbf{M}_{\widehat{R}:c_{\widehat{r}}} $.
which concludes $\beta_{\widehat{r}+1}$ is nonzero, so we can simply assume it is $-1$.
Then 
\begin{align*}
 \beta_1 \mathbf{M}_{\widehat{R}:c_1} + ... + \beta_{\widehat{r}} \mathbf{M}_{\widehat{R}:c_{\widehat{r}}}   =  \mathbf{M}_{\widehat{R} : i} 
\hspace{5mm} \implies  \hspace{5mm}
 \beta_1 \mathbf{M}_{R:c_1} + ... + \beta_{\widehat{r}} \mathbf{M}_{R:c_{\widehat{r}}}   =  \mathbf{M}_{R : i}
\end{align*}
Due to uniqueness of $\alpha_j$'s above, we can tell that 
\begin{align*}
    \alpha_1 = \beta_1 \hspace{10mm} \alpha_2 = \beta_2 \hspace{10mm} \ldots   \hspace{10mm} \alpha_{\widehat{r}} = \beta_{\widehat{r}}  \hspace{10mm} \alpha_{\widehat{r}} = \beta_{\widehat{r}}
\end{align*}
Then the vector
$y_{\widehat{R} }=\alpha_1 \mathbf{M}_{\widehat{R}:c_1} + \ldots + \alpha_{\widehat{r}} \mathbf{M}_{\widehat{R}:c_{\widehat{r}}}   -  \mathbf{M}_{\widehat{R} : i}  = 0$ is a zero vector.
However it is a contradiction because if $y_{\widehat{R}}$ is zero vector  then $y_a=0$ due to $a\in \widehat{R}$ which we already know $y_a\neq 0$.\medskip \\
Therefore, being nonzero of $y_a$ implies non-singularity of $\mathbf{M}_{\widehat{R}:\widehat{C}}$ which is equivalent to the detection of the independence of column $\mathbf{M}_{:i}$ due to lemma 2.
As a conclusion, probability of detection of independence of an active column is at least $\frac{k}{m-observed}$  and considering the fact that $observed \geq j$ it follows that  $\frac{k}{m-observed} > \frac{k}{m-j}$ and it give the final conclusion of the desired probability is lower bounded by:
$\frac{k}{m-j}$. As desired.
\end{proof}
\bigskip
\textit{Step 4 :} We can model execution of $\mathbf{ERR}$ as following stochastic process: 
\begin{align*}S_0= X_{0,1} + X_{0,2} + . . . + X_{0,n}
\end{align*}
where each of the $X_{0,j}$ corresponds to the indicator variable of the activeness of the column $\mathbf{M}_{:j}$.
Obviously, initially at least $r$ of these random variables are equal to 1. 
We define $S_1$ similarly:
\begin{align*}S_1= X_{1,1} + X_{1,2} + . . . + X_{1,n}
\end{align*}
and for any j that $X_{0,j}=1$ satisfied, at this phase $X_{1,j}$ will be equal to 0 with probability at least $\frac{k}{m-0}$ from lemma \ref{lemma:prob_bound}. 
For remaining $j$'s that $X_{0,j}=0$ satisfied then $X_{1,j}=0$ also to be satisfied.
For the next step $S_2$ defined as:
$$S_2= S_1 +  X_{2,1} + X_{2,2} + . . . + X_{2,n_2}$$ 
where again  for any $j$ that $X_{0,j}=1$ satisfied, at this phase $X_{1,j}$ will be equal to $0$ with probability at least $\frac{k}{m-1}$ from lemma \ref{lemma:prob_bound}.
Remaining $j$'s will stay as $X_{2,j}$ to be equal to 0.
In general 
\begin{align*}S_{iter} = X_{iter,1} + X_{iter,2} + . . . + X_{iter,n_2} 
\end{align*}
where again  for any j that $X_{iter-1,j}=1$ satisfied, at this phase $X_{iter,j}$ will be equal to 0 with probability at least $\frac{k}{m-(iter-1)}$ from lemma \ref{lemma:prob_bound}.
The termination of 
algorithm is equivalent to the point $S_p = 0$ in this model.
One can see termination of this process is upper bounded by termination of the 
following process :
\begin{align*}S'_0 = X'_{0,1} + X'_{0,2} + . . . + X'_{0,r}
\end{align*}
where each of the $X'_{0,j}$ is set to be equal to $1$. we define $S'_1$ in a similar way:
\begin{align*}S'_1 = X'_{1,1} + X'_{1,2} + . . . + X'_{1,r}
\end{align*}
where each of $X'_{1,j}$ is equal to $0$ with probability $\frac{k}{m}$. Then:
\begin{align*}S'_2 = X'_{2,1} + X'_{2,2} + . . . + X'_{2,r}.
\end{align*}
Similarly $X'_{2,j}$ is set to be $0$ if $X'_{1,j}=0$ and $X'_{2,j}$ is equal to $0$ with probability $\frac{k}{m-1}$ otherwise.
In general:
\begin{align*}S'_{iter} = X'_{iter,1} + X'_{iter,2} + . . . + X'_{iter,r} 
\end{align*}
again $X'_{iter,j} = 0$ if $X'_{iter-1,j} = 0$ and, $X'_{iter,j}=0$ with probability $\frac{k}{m-(iter-1)}$ otherwise.\\\\\\
\textit{Step 5:} \hypertarget{step5}{Here}  we use a combinatorial argument to bound number of observation in each column.
\begin{lemma}
Let $X'$ be a process that is zero initially: $X'_0 = 1$ and remaining entries defined as 
\begin{align*}
    X'_{i+1} = 
    \begin{cases}
    \begin{cases}
        0 & \text{with probability } \frac{k}{m-i} \\
        1 & \text{otherwise}
    \end{cases}    & \hspace{3mm} \text{if  } \hspace{3mm}  X'_i = 1\\
    0   & \hspace{3mm}  \text{if  } \hspace{3mm}  X'_i = 0
    \end{cases}
\end{align*} 
Then expected point that $X'$ to switch to 0 is $\frac{m+1}{k+1}$.
\end{lemma}

\begin{proof}
Lets denote the expected switch time with $st$ and write the expression for it: 
\begin{align*}
\mathbb{E}[st] = \sum i P(st = i) =  1 \frac{k}{m} + 2 \frac{k}{m-1}\Big(1-\frac{k}{m}\Big) + 3\frac{k}{m-2}\Big(1-\frac{k}{m}\Big)\Big(1-\frac{k}{m-1}\Big) + \dots
\end{align*}
We claim that this sum is equal to the expected position of the first $1$ in a random binary string with $k$ many $1$ and $m-k$ many $0$.
To observe truth of the claim we notice followings:
\begin{itemize}
    \item First $1$ being in the first position is obviously $\frac{k}{m}$ as there are $k$ many $1$'s out of $m$ many characters.
    \item The probability of the first $1$ being in the second place is $(1-\frac{k}{m})\frac{k}{m-1}$. The first entry being zero has probability: $1-\frac{k}{m}$ and the second entry being one is $\frac{k}{m-1}$
    \item The probability of the first $1$ being in the $i$-th place is 
    $$\Big(1-\frac{k}{m}\Big)\Big(1-\frac{k}{m-1}\Big)\ldots \Big(1-\frac{k}{m-(i-1)}\Big) \Big( \frac{k}{m-(i-1)}\Big).$$ The first entry being zero has probability: $1-\frac{k}{m}$, the second entry being zero has probability $1-\frac{k}{m-1}$ and so on so forth. Finally out of remaining $m-i+1$ entries the next one being $1$ is equal to $\frac{k}{m-(i-1)}$.
\end{itemize}
Then expected position of the first 1 is equal to 
\begin{align*}
 1 \frac{k}{m} + 2 \frac{k}{m-1}\Big(1-\frac{k}{m}\Big) + 3\frac{k}{m-2}\Big(1-\frac{k}{m}\Big)\Big(1-\frac{k}{m-1}\Big) + \ldots   
\end{align*}
which is equal to $\mathbf{E}[st]$.
Lets find the position of the first $1$ by double counting technique. 
A word with $k$ number of $1$ and $m - k$ number of $0$ 
can be represented as $a_0 1 a_1 1 a_2 . . . 1 a_k$ where $a_i$ represents number 
of zeros between two $1$'s. 
Now, lets find number of first 1 in the $k+1$ sized set of following words
\begin{align*}
& a_0 1 a_1 1 a_2 . . . 1 a_k,  \\
& a_1 1 a_2,...,a_k 1 a_0, \\
& a_2 1 a_3,...,a_0 1 a_1, \\
& \vdots \\
& a_k 1 a_0,...,a_k 1 a_0 
\end{align*}
Expected number of first 1 here is simply \medskip 
\begin{align*}
\frac{a_0+1}{k+1} + \frac{a_1+1}{k+1} + \ldots +\frac{a_k+1}{k+1} =  \frac{a_0+a_1+ ... +a_k + k+1}{k+1}   = \frac{m+1}{k+1}.
\end{align*} \medskip
So, we can divide set of all words with $k$ many $1$'s and $m-k$ many $0$'s into $k+1$-sized sets.
For each group the average position of the first 1 will be $\frac{m+1}{k+1}$.
Therefore, in overall the average position of the first $1$ is $\frac{m+1}{k+1}$.
\end{proof}
\hspace{-5mm}A simple followup of this lemma is  to notice:
$$\mathbb{E}[st]=\frac{m+1}{k+1}< \frac{m}{k}$$  due to $m>k$. 
Then, we can use the Markov inequality to get: $$P\Big(st>2\frac{m}{k}\Big) < \frac{1}{2}.$$
Moreover, from the combinatorial counting argument we can imply that the probability of $st > a$ will be given as 
\begin{align*}
P(st > a) = \frac{ \binom{m-a}{k} } { \binom{m}{k} }
\end{align*}
using the previous inequality we can observe that:
\begin{align*}
P\Big(st > \frac{2m}{k}\Big) = \frac{ \binom{m-2m/k }{k} } { \binom{m}{k} } < \frac{1}{2}
\end{align*}
Considering the fact 
\begin{align*}
f(x) = \frac{ \binom{x-2m/k}{k} } { \binom{x}{k} }
\end{align*}
is an increasing function and
\begin{align*}
P\Big(st > \frac{\alpha m}{k}\Big) = 
\frac{ \binom{m-2m/k }{k} } { \binom{m}{k} } 
\frac{ \binom{m-4m/k }{k} } { \binom{m-2m/k}{k} }
\cdots
\frac{ \binom{m-2 \alpha m/k }{k} } { \binom{m-2(\alpha-1)m/k}{k} }
< (\frac{1}{2})^\alpha 
\end{align*}
For a given $\epsilon$, if we set $\alpha = \log{\frac{1}{\epsilon}}$ we conclude that with probability at least $1-\epsilon$ the following inequality satisfied:
\begin{align*}
st > 2 \frac{m}{k} \log{\frac{1}{\epsilon}}.    
\end{align*}
\\
\textit{Step 6:} So, we can tell 
\begin{align*}
P\Big(X' \geq 2 \log{(\frac{1}{\epsilon})} \frac{m}{k}\Big) \leq \epsilon.    
\end{align*}
Which means for a given $j$, with probability more than $1-\epsilon$,  $X'_{i,j}$ will switch to zero before   $ 2 \log(\frac{1}{\epsilon})\frac{m}{k}$ for any $ j \in [r]$. 
Using union bound argument, after $2\log(\frac{1}{\epsilon})\frac{m}{k}$ 
iteration with probability more than $1-\epsilon r$, for any $i\in [r]$, $X'_{i,j}$ will switch to zero.\\\\
Therefore, the process $S$ will stop before $2\log{\frac{r}{\epsilon}}\frac{m}{k}$ iteration with probability $1-\epsilon$. 
Remind that, termination time of $S$ corresponds to the value of $T$ and number of total red points is bounded by $Tn$.
Then number of total red observations is bounded by: $$2 \frac{m n}{k} \log{\frac{r}{\epsilon}}.$$
Finaly, total number of observations is equal to the number of red observations plus number of blue observations which gives the bound:
\begin{align*}
(m+n-r)r+  2 \frac{m n}{k} \log{\frac{r}{\epsilon}}. 
\end{align*}
\end{proof}
\hspace{-6mm}To translate this result to coherence number rather than \textit{space sparsity number}, we use the following lemma:
\begin{lemma}  \label{cohbd}
Let $\mathbb{U}$ be an $r$-dimensional subspace of $\mathbb{R}^{m}$. Then the below relation between $\psi(\mathbb{U})$ and $\mu(U)$  holds:
\begin{align*}
\mu(U) \geq \frac{m}{r} \frac{1}{\psi(\mathbb{U})}.
\end{align*}
\end{lemma}

\begin{proof}
We again denote $\psi(\mathbb{U})$ with $k$ for ease of reading.
By the definition of the 
\textit{space sparsity number}, we see that there exists a vector $v\in U$ and $k$ different indices $i_1,i_2,...,i_k$ 
such that the only nonzero components of $v$ are $v_{i_1},v_{i_2},...,v_{i_k}$. 
Up to scaling, we may assume that $v$ is 
a unit vector. 
This is equivalent to  
\begin{align*}
 {v_{i_1}}^2 + ... + {v_{i_k}}^2 = 1   
\end{align*}
Therefore, we observe that there is an index $i_a$ satisfies ${v_{i_a}}^2 \geq \frac{1}{k}$. 
If this was not the case, then for all $j$ with $1\leq j \leq k$,  ${v_{i_j}}^2 < 
\frac{1}{k}$ should satisfy, and this implies 
$$1={v_{i_1}}^2 + ... + {v_{i_k}}^2 < k \frac{1}{k} = 1$$
and this is a contradiction. 
Using these facts, we can see that 
\begin{align*}
 || P_U e_{i_a} ||^2 \geq || v \cdot e_{i_a} ||^2 = | v \cdot e_{i_a} |^2 = {v_{i_a}}^2 \geq \frac{1}{k}   
\end{align*}
where $e_{i_a}$ is $i_a$'th standard basis of $\mathbb{R}^{m}$. 
The first inequality follows from the fact that the length of projection of any vector to the subspace 
$\mathbb{U}$ is always greater or equal than the length of the projection onto a vector of that subspace. 
Thus, we have 
\begin{align*}
\mu(U) = \frac{m}{r} \underset{1 \leq j \leq m}{\max}  || P_U e_{j}||^2 
\geq  \frac{m}{r}|| P_U e_{i_a}||^2 \geq \frac{m}{r} \frac{1}{k}
= \frac{m}{r} \frac{1}{\psi(\mathbb{U})}    
\end{align*}
\end{proof}

\subsection{Discussion for Incoherent Row Spaces:}
In the lemma \ref{cohbd} we show that $$\mu(\mathbb{U}) \geq \frac{m}{r} \frac{1}{\psi(\mathbb{U})}.$$ and in the theorem above we prove that the observation complexity of $\mathbf{ERR}$ is upper bounded by $(m+n-r)r + 2 \frac{m n}{\psi(\mathbb{U})} \log{\frac{r}{\epsilon}}$ where $\mathbb{U}$ is column space of the matrix $\mathbf{M}$. \\\\
Lets denote the fraction $$\gamma = \frac{m}{\psi(\mathbb{U})} \frac{1}{\mu(\mathbb{U}) r}$$ then lemma \ref{cohbd} is equivalent to $\gamma \leq 1 $.
Lets transfer observation complexity of $\mathbf{ERR}$ with respect to $\mu(\mathbb{U})$ using $\gamma$.
Then we get the observation complexity is $$(m+n-r)r + 2\gamma \mu(\mathbb{U}) r \log{r/\epsilon}$$ and using the fact that $\gamma \leq 1$ this number is smaller than bound due to \cite{nina}:
$$(m+n-r) + 2 \mu(\mathbb{U}) r \log{r/\epsilon}$$
In many cases $\gamma$ can be very small. 
For any matrix that has high value of-$\psi(\mathbb{U})$ or low value of $\mu(\mathbb{U})$,  $\gamma$ is guaranteed to be very small. 
Specifically, if $\psi(\mathbb{U})$ is $\Theta(m)$ or $\mu(\mathbb{U})$ is $\Theta{\frac{m}{r}}$ then $\gamma$ is $\mathcal{O}(\frac{1}{r})$.
Proofs for each case provided below:\\\\
\textit{$\psi(\mathbb{U})$ is $\Theta(m)$}:  Assigning $\psi(\mathbb{U})$ being $\Theta(m)$ in the definition of $\gamma$, we conclude that $\gamma$ is $\Theta(\frac{1}{\mu(U)r})$.
Remember from the definition of the coherence, $\mu(\mathbb{U}) \geq 1$ for any subspace, which gives the final conclusion of $\gamma$ is $\mathcal{O}(\frac{1}{r})$. \medskip\\
\textit{$\mu(\mathbb{U})$ is $\Theta{\frac{m}{r}}$}:  Assigning $\mu(\mathbb{U})$ being $\Theta(\frac{m}{r})$ in the definition of $\gamma$, we conclude that $\gamma$ is $\Theta(\frac{1}{\psi(\mathbb{U})})$.
Moreover, remember that from lemma \ref{lem:bds}, we know that $\psi(\mathbb{U})$ is $\Omega(r)$ which gives final conclusion of $\mathcal{O}(\frac{1}{r})$. \medskip\\

\subsection{Coherent Row Spaces}

\begin{theorem*}[ Coherent row space]  
Let $r$ be the rank of underlying $m\times n$ sized matrix $\mathbf{M}$ with column space $\mathbb{U}$ and row space $\mathbb{V}$. 
Then,  \hyperlink{err}{$\mathbf{ERR}$} exactly recovers the underlying matrix $\mathbf{M}$ with probability at least $1-\epsilon$  using at most 
$$(m+n-r)r + \frac{\frac{2m}{\psi(\mathbb{U})}\big(r+2 +\log{\frac{1}{\epsilon}}\big)}{\psi(\mathbb{V})}n $$
observations.
\end{theorem*}

\begin{proof}%[\bf Proof] 
We use the same terminology as previous theorem and $k$ and $t$  stands for $\psi(\mathbb{U})$ and $\psi(\mathbb{V})$ correspondingly. 
So, if a column is not in the column space of $C$ then we call it active.\medskip\\
From lemma \ref{lemma:prob_bound}, we know that at any step if a column is still active, then probability of its detection is at least $\frac{k}{m}$ where $k$ is the \textit{space non-sparsity number} for column space.
Let's just focus on active observations, and estimate the number of required active observations to detect $r$-th linearly independent column.
We can see that, under the condition of each observation being active observation and the probability of detection being exactly $\frac{k}{m}$ the process of the detection of $r$-th independent column can be modelled as negative binomial distribution.\medskip\\
Lets remind the formula of the probability mass function negative binomial distribution as getting $a$-th success in the $a+b$'th step while success probability being $p$ :
$$ f(a,b,p) = \binom{a+b-1}{a}p^a (1-p)^b$$
For this problem, we are interested to find the probability for finding $r$-th success at $N$-th trial
which corresponds to :
$$ f(r,N-r,\frac{k}{m}) = \binom{N-1}{r}{ \Big( \frac{k}{m}\Big) }^r \Big( 1- \frac{k}{m}\Big) ^{N-r-1}$$
As the number of observations is the focus of this theorem, we fix parameters $k,m,r$ and investigate the behaviour of the function while $N$ being variable.
Intuitively, we use the following notation: 
$$\tau_{k,m,r}(N) =  f(r,N-r,\frac{k}{m})$$
In lemma \ref{lm:taubd} and \ref{1/n} we investigate properties of this function to have better understanding of failure probability of $\mathbf{ERR}$: \\
\begin{lemma} \label{lm:taubd}
$\tau_{k,m,r}(N)$ is a decreasing function after N being larger than $(\frac{2m}{k}+1) r$. Specifically,
we can give the following bound for the decreasing rate: 
$$ 1-\frac{k}{m} < \frac{\tau_{k,m,r}(N+1)}{\tau_{k,m,r}(N)} < 1-\frac{k}{2m} $$
\end{lemma}
\begin{proof}
To show the decreasing we analyse the fraction : \\
\begin{align*}
  \frac{\tau_{k,m,r}(N+1)}{\tau_{k,m,r}(N)}  = \frac{ \binom{N}{r}{ \Big( \frac{k}{m}\Big) }^r \Big( 1- \frac{k}{m}\Big) ^{N-r} }
{\binom{N-1}{r}{ \Big( \frac{k}{m}\Big) }^r \Big( 1- \frac{k}{m}\Big) ^{N-r-1} } 
&=\frac{ \frac{N!}{r!(N-r)!}{ \Big( \frac{k}{m}\Big) }^r \Big( 1- \frac{k}{m}\Big) ^{N-r} }{\frac{(N-1)!}{r!(N-1-r)!}{ \Big( \frac{k}{m}\Big) }^r \Big( 1- \frac{k}{m}\Big) ^{N-r-1}}\\[0.7ex]
&=\frac{N}{N-r} (1-\frac{k}{m})
\end{align*}
So, we get following recursive formula:
\begin{align*}
\tau_{k,m,r}(N+1)  =\frac{N}{N-r} \Big(1-\frac{k}{m}\Big){\tau_{k,m,r}(N)}.    
\end{align*}
Left side of the the target inequality is easy to prove as $\frac{N}{N-r}>1$ implies
$$ \frac{\tau_{k,m,r}(N+1)}{\tau_{k,m,r}(N)}  > 1-\frac{k}{m}. $$
Then, we only need to prove the right side of the inequality.
Lets make the following observations  $$\frac{N}{N-r} = 1 + \frac{r}{N-r}$$
and from the hypothesis of the lemma we have $$N > \Big(\frac{2m}{k}+1\Big)r  \implies N-r > \frac{2m}{k}r \implies \frac{r}{N-r} < \frac{k}{2m}. $$
Now, we are ready to prove rigth side:\\
\begin{align*}
\frac{\tau_{k,m,r}(N+1)}{\tau_{k,m,r}(N)}  = \frac{N}{N-r}\Big(1-\frac{k}{m}\Big) 
&= \Big(1+\frac{r}{N-r}\Big)\Big(1-\frac{k}{m}\Big)  \\
&< \Big(1+\frac{k}{2m}\Big)\Big(1-\frac{k}{m}\Big)   \\
& = 1-\frac{k}{2m}-\frac{k^2}{2m^2}  \\
& < 1-\frac{k}{2m}.
\end{align*}
 Therefore:\\
 \begin{align*}
  1-\frac{k}{m} < \frac{\tau_{k,m,r}(N+1)}{\tau_{k,m,r}(N)} < 1-\frac{k}{2m}.    
 \end{align*}
 Note that we can claim decreasing of $\tau_{k,m,r}$ just follows from the right side of the inequality.
\end{proof}
To explore more properties of the function $\tau_{k,m,r}$ we prove the following lemma.

\begin{lemma} \label{1/n}
Lets assume $n$ is a positive integer. Then $\tau_{k,m,r}$ satisfies the following inequality 
\begin{align*}
 \tau_{k,m,r}\Big(\frac{2m}{k}(r+1)+n\Big) \leq \frac{1}{n}.   
\end{align*}
\end{lemma}
\begin{proof}
It is clear that  $\tau_{k,m,r}\Big(\frac{2m}{k}(r+1)\Big) < 1$ as it is value of a probability mass function.
In lemma 3 we proved that the functions $\tau_{k,m,r}$ is decreasing after $\frac{2m}{k}(r+1)$.
Therefore, for any positive integer $n$ the following inequalities satisfied:
\begin{align*}
\tau_{k,m,r}\Big(\frac{2m}{k}(r+1)+n\Big) &< \tau_{k,m,r}\Big(\frac{2m}{k}(r+1)+n-1\Big) \\
\tau_{k,m,r}\Big(\frac{2m}{k}(r+1)+n\Big) &< \tau_{k,m,r}\Big(\frac{2m}{k}(r+1)+n-2\Big) \\
                               &\vdots \\
\tau_{k,m,r}\Big(\frac{2m}{k}(r+1)+n\Big) &< \tau_{k,m,r}\Big(\frac{2m}{k}(r+1)\Big) 
\end{align*}
By summing all these inequalities we conclude:
\begin{align*}
   n \tau_{k,m,r}\Big(\frac{2m}{k}(r+1)+n\Big) < \sum_{i=1}^n \tau_{k,m,r}\Big(\frac{2m}{k}(r+1)+i\Big) 
\end{align*}
To bound the second term, we can use: $$\sum_{i=1}^n \tau_{k,m,r}\Big(\frac{2m}{k}(r+1)+i\Big) \leq  \sum_{i=r}^{\infty}\tau_{k,m,r}(i) = 1 $$
and dividing left and rigth side of the inequality above concludes:
\begin{align*}
    n \tau_{k,m,r}\Big(\frac{2m}{k}(r+1)+n\Big) < 1.
\end{align*}
\end{proof}
To apply the lemma above for $n = \frac{2m}{k}$ we get, $$\tau_{k,m,r}\Big(\frac{2m}{k}(r+1)+\frac{2m}{k}\Big) < \frac{k}{2m}$$
Using right side of the lemma \ref{lm:taubd} we notice :
$$\tau_{k,m,r}\Big(\frac{2m}{k}(r+1)+\frac{2m}{k} + i\Big)< \frac{k}{2m}\Big(1-\frac{k}{2m}\Big)^i$$
for any positive integer $i$. Picking $i = \frac{2m}{k} \log{\frac{1}{\epsilon}}$ follows as :
\begin{align*}
 \tau_{k,m,r}\Big(\frac{2m}{k}(r+1)+\frac{2m}{k} +  \frac{2m}{k} \log{\frac{1}{\epsilon}} \Big)  &< \frac{k}{2m}  \Big(1-\frac{k}{2m}\Big)^{\frac{2m}{k} \log{\frac{1}{\epsilon}}}\\[0.5ex]   
&<  \frac{k}{2m}  e^{- \log{\frac{1}{\epsilon}}}  
=  \frac{k}{2m}  \epsilon  
\end{align*}
second inequality here is application of the $(1- \frac{1}{\alpha})^{\alpha} < \frac{1}{e}$ for $\alpha > 0$. Therefore we currently have :
$$ \tau_{k,m,r}\Big(\frac{2m}{k}(r+1)+\frac{2m}{k} +  \frac{2m}{k} \log{\frac{1}{\epsilon}}\Big)  <  \frac{k}{2m}  \epsilon  $$
and we target to bound :
$$ \sum_{i=0}^{\infty} \tau_{k,m,r}\Big(\frac{2m}{k}(r+1)+\frac{2m}{k} +  \frac{2m}{k} \log{\frac{1}{\epsilon}} + i \Big) .  $$
To apply right side of lemma \ref{lm:taubd}, $i$ times we conclude :\\
\begin{align*}
 \tau_{k,m,r}\Big(\frac{2m}{k}(r+1)+\frac{2m}{k} +  \frac{2m}{k} \log{\frac{1}{\epsilon}} + i \Big) &<\\ &\tau_{k,m,r}\Big(\frac{2m}{k}(r+1)+\frac{2m}{k} +  \frac{2m}{k} \log{\frac{1}{\epsilon}} \Big)\Big(1-\frac{k}{2m}\Big)^i
\end{align*}\\
Therefore the summation above can be upper bounded as: 
\begin{align*}
 \sum_{i=0}^{\infty} \tau_{k,m,r}\Big(\frac{2m}{k}(r+1)+\frac{2m}{k} +  &\frac{2m}{k} \log{\frac{1}{\epsilon}} + i \Big)    <\\ 
 &<\sum_{i=0}^{\infty}  \tau_{k,m,r}\Big(\frac{2m}{k}(r+1)+\frac{2m}{k} +  \frac{2m}{k} \log{\frac{1}{\epsilon}} \Big)\Big(1-\frac{k}{2m}\Big)^i  \\
&= \tau_{k,m,r}\Big(\frac{2m}{k}(r+1)+\frac{2m}{k} +  \frac{2m}{k} \log{\frac{1}{\epsilon}} \Big) \sum_{i=0}^{\infty} \Big(1-\frac{k}{2m}\Big)^i  \\
&= \tau_{k,m,r}\Big(\frac{2m}{k}(r+1)+\frac{2m}{k} +  \frac{2m}{k} \log{\frac{1}{\epsilon}} \Big) \frac{2m}{k} \\
&< \epsilon \frac{k}{2m}  \frac{2m}{k}  = \epsilon.
\end{align*}
Therefore, we conclude that the probability of $\mathbf{ERR}$ terminating after  $\frac{2m}{k}\big(r+2 +\log{\frac{1}{\epsilon}}\big)$ is smaller than $\epsilon$.\\\\
At this point we have number upper bound for number of active observations in order to have $1-\epsilon$ probability of termination.
However, we need to give the bound with respect to number of overall observations.
Following lemma will help us for that purpose 

\begin{lemma} \label{lem:activecolumns}
At every phase of the algorith-$\mathbf{ERR}$, if there is at least one active observation, then there is at least $t$ many active observations.
\end{lemma}
\begin{proof} 
The first step is to observe that, any column in $C$ is already inactive as they are already in temporary column space.
The second observation is any column that is linear combination of columns in C also already inactive.
We prove the lemma by assuming the hypothesis of the lemma is not correct and we will deduce contradiction from that.
Therefore, we assume that there is a step that the number of active columns is less than $t$, under the condition not all columns are inactive.\\\\
Number of active columns  being smaller than $t$ implies that the number of inactive columns is larger than $n-t$.
Which implies there is a subset of columns- $\Omega'$ that satisfies $|\Omega'|>n-t$ and $\mathbf{M}_{:\Omega'}$ has rank of at most $r-1$ (as there are still some active columns).\\\\
We know that the rank of $\mathbf{M}$ being $r$ implies there is at least one set of $r$ many linearly independent rows.
Lets denote one of these sets by $R=\{j_1,j_2,...,j_r\}$ and naturally, the set of row vectors
$\mathbf{M}_{j_1:}, \mathbf{M}_{j_2:},..., \mathbf{M}_{j_r:}$ are linearly dependent.\\\\
Returning back to the argument $M_{:\Omega'}$ having a rank of at most $r-1$, implies the rank of $M_{R:\Omega'}$ is also at most $r-1$.
Therefore, there is a linear dependence relation among the vectors $\mathbf{M}_{j_1:\Omega'}$, $\mathbf{M}_{j_2:\Omega'}$, . . . ,$\mathbf{M}_{j_r:\Omega'}$. 
As we already have $\Omega'>n-t$ then using lemma 1 we conclude that there is linear dependence relation among $\mathbf{M}_{j_1:}, \mathbf{M}_{j_2:},..., \mathbf{M}_{j_r:}$ which is a contradiction.
Therefore, if there is one active column we can conclude there is at least $t$ many active columns.
\end{proof}
Rest of the proof is simple counting argument.
We know that if we have $\frac{2m}{k}\big(r+2 +\log{\frac{1}{\epsilon}}\big)$ many observations then with probability larger than $1-\epsilon$ our algorithm succeeds.
Moreover, from the lemma above, as at each phase we have at least $\psi(\mathbb{V})$ many observations, $$\frac{\frac{2m}{k}\big(r+2 +\log{\frac{1}{\epsilon}}\big)}{t}$$ many phase is enough to have desired number of active observations.
Note that, at each step we have at most n many observation, which concludes the statement
$$\frac{\frac{2m}{k}\big(r+2 +\log{\frac{1}{\epsilon}}\big)}{t}n$$ many observation is enough to guarantee with probability $1-\epsilon$
\end{proof}

\subsection{Proof of corollary \ref{cor:err} }

We start by rephrasing the corollary 5 and prove the statement for each case later on.
\begin{corollary*} 
Observation complexity of $\mathbf{ERR}$ studied for three different case below:
\begin{itemize}
    \item if  $ \psi(\mathbb{V})=\mathcal{O}(1)$ then observation complexity is  upper bounded by $(m+n-r)r+2 \frac{m n}{\psi(\mathbb{U})}\log{(\frac{r}{\epsilon})}\\=(m+n-r)r + \mathcal{O}\big(nr\mu_0\log{(\frac{r}{\epsilon})}\big)$.
    ( this bound matches with \cite{nina} but many times it is much smaller quantity as we discussed in previous section)
\vspace{-2mm}
    \item  if  $ \psi(\mathbb{V})=\Theta(r)$ then observation count is upper bounded by $(m+n-r)r+   \mathcal{O}\Big(\frac{\frac{2m}{\psi(\mathbb{U})}(r+2 +\log{\frac{1}{\epsilon}})}{r}n\Big) \\=
(m+n-r)r + \mathcal{O}\big(n \mu_0(r+\log{\frac{1}{\epsilon}}) \big) $. Selecting $\epsilon = \frac{1}{2^{\mathcal{O}(r)}}$ gives bound of  $mr + \mathcal{O}(n \mu_0r)$
\vspace{-2mm}
    \item if  $ \psi(\mathbb{V})=\Theta(n)$ then observation count is upper bounded by  $(m+n-r)r+  \mathcal{O}\Big(\frac{\frac{2m}{\psi(\mathbb{U})}(r+2 +\log{\frac{1}{\epsilon}})}{n}n\Big) \\ =
(m+n-r)r +  \mathcal{O}\big( \mu_0 r(r+\log{\frac{1}{\epsilon}}) \big) $ Selecting $\epsilon = \frac{1}{2^{\mathcal{O}(r)}}$ gives bound: $\mathcal{O}((m+n-r)r)$

%    2 \frac{m n}{k}\log{(\frac{r}{\epsilon})}=(m+n-r)r +
%    \frac{\frac{2m}{k}(r+2 +\log{\frac{1}{\epsilon}})}{t}n
%    \mathcal{O}(mr\mu_0\log{(\frac{r}{\epsilon})})$

\end{itemize}
\end{corollary*}

\begin{proof}
\textit{Case} : $ \psi(\mathbb{V})=\mathcal{O}(1)$.
From the theorem \ref{thm:lg2} the observation complexity is upper bounded by $$(m+n-r)r +  \mathrm{min}\Big(  2 \frac{m n}{{\psi}(\mathbb{U})}\log{(\frac{r}{\epsilon})} , \frac{\frac{2m}{\psi(\mathbb{U})}(r+2 +\log{\frac{1}{\epsilon}})}{\psi(\mathbb{V})}n \Big)  $$
therefore it is upper bounded by $(m+n-r)r+2 \frac{m n}{\psi(\mathbb{U})}\log{(\frac{r}{\epsilon})}$.
Moreoover, in lemma \ref{cohbd} we show $$\mu(\mathbb{U}) \geq \frac{m}{r} \frac{1}{\psi(\mathbb{U})}$$ which upper bounds the last quantity by 
$(m+n-r)r + \mathcal{O}\big(nr\mu_0\log{(\frac{r}{\epsilon})}\big)$. \\\\
\textit{Case}  $ \psi(\mathbb{V})=\Theta(r)$: This time we choose the second term in $\mathrm{min}$ operator of theorem \ref{thm:lg2}. 
We note that $\frac{m}{\psi(\mathbb{U})}$ can be upper bounded by $\mu(\mathbb{U})r$ and plugging it together with $\psi(\mathbb{V})=\Theta(r)$ gives us upper bound of $(m+n-r)r + \mathcal{O}\big(n \mu_0(r+\log{\frac{1}{\epsilon}}) \big) $. 
Moreover, if  $\epsilon = \frac{1}{2^{\mathcal{O}(r)}}$ then $\log{\frac{1}{\epsilon}}$ is $\mathcal{O}(r)$, therefore right summand is bounded by  $\mathcal{O}(n \mu_0r)$. Considering the fact $\mu_0 \geq 1$ always, then overall expression is upper bounded by $mr + \mathcal{O}(n \mu_0r)$
\\\\
\textit{Case}  $ \psi(\mathbb{V})=\Theta(n)$: This case is just similar too previous case with the difference of plugging  $\psi(\mathbb{V})=\Theta(n)$ gives us the bound of $(m+n-r)r +  \mathcal{O}\big( \mu_0 r(r+\log{\frac{1}{\epsilon}}) \big)$. 
Using the similar bound to $\epsilon$ makes the right summand to be  $\mathcal{O}(\mu_0 r^2)$.
Moreover from the definition of coherence we have $\mu_0 \leq \frac{m}{r}$ which upper bounds this term by $\mathcal{O}(m r)$ therefore overall sum is upper bounded by $\mathcal{O}((m+n-r)r)$.
\end{proof}
%\todo{$\Theta$ and big O and omegani izah ele notationsda, pseudo inversi de, algorithmlere goz gezdir, mu0-lar ve algo statemntler, woodrufun costly recovery problemine de el at, refer falan}

\newpage

\section{Proof of Theorem \ref{thm:erre}. Exact Recovery While Rank Estimation}

We start with rephrasing the theorem 4. Then we prove the theorem statement and its corollary.

\begin{theorem*}  (Exact Recovery while Rank Estimation)
Let $r$ be the rank of underlying $m\times n$ sized matrix $\mathbf{M}$ with column space $\mathbb{U}$ and row space $\mathbb{V}$. 
Then, \hyperlink{erre}{$\mathbf{ERRE}$} exactly recovers the underlying matrix $\mathbf{M}$ while estimating rank with probability at least $1- ( \epsilon + e^{-T\frac{\psi(\mathbb{U})\psi(\mathbb{V})}{m}})$  using at most 
\begin{align*}
  (m+n-r)r+Tn +  \mathrm{min} \Big(  2 \frac{m n}{\psi(\mathbb{U})}\log{(\frac{r}{\epsilon})} , \frac{\frac{2m}{\psi(\mathbb{U})}(r+2 +\log{\frac{1}{\epsilon}})}{\psi(\mathbb{V})}n ) \Big)     
\end{align*}
observations.
\end{theorem*}

\begin{proof}
We again use $k$ and $t$ for $\psi(\mathbb{U})$ and $\psi(\mathbb{V})$ correspondingly and use all the terminology from the previous proofs. 
Then, we start by proving that under the scenario there is still active column, then with probability $1-e^{-T \frac{kt}{m}}$, it will be detected in $T$ phases.
We prove the following key lemma in order to accomplish the proof of the theorem.

\begin{lemma}
Lets assume the underlying matrix $\mathbf{M}$ has row \textit{space non-sparsity number} $k$ and column \textit{space non-sparsity number} $t$. 
Then, if at an intermediate step of $\mathbf{ERRE}$ still column space not recovered completely, then with probability $1-e^{-T \frac{kt}{m}}$ new independent column will be detected within $T$ phases.
\end{lemma}

\begin{proof}
For every active column observation, the probability of detecting independence is at least $1-\frac{k}{m}$ from the lemma \ref{lemma:prob_bound}. 
From the lemma~\ref{lem:activecolumns} , if there is one active column, then there is at least $t$ many active column in that phase.
Therefore, the probability of detection of an active column is at least
$$\Big(1-\frac{k}{m}\Big)^t.$$
Then, we conclude that after $T$ many phase, detection probability is at least
$$\Big(1-\frac{k}{m}\Big)^{t T}.$$ 
Using the inequality $1+ x \leq e^x$ for $\forall x \in \mathbb{R}$ the quantity above can be bounded by:
$$\Big(1-\frac{k}{m}\Big)^{t T} < e^{-T\frac{kt}{m} }.$$
%Plugging $T = \frac{m}{kt} \log{\frac{1}{\epsilon}}$ we can bound
%$$e^{-\frac{k}{m}t T} = e^{-\frac{k}{m}t \frac{m}{kt} \log{\frac{1}{\epsilon}}} = e^{-\log{\frac{1}{\epsilon}}} %= e^{\log{\epsilon}}=\epsilon. $$
%Which gives us the conclusion, after $\frac{m}{kt}\log{\frac{1}{\epsilon}}$ many phase, the probability of the detection of active column is smaller than $\epsilon$.
\end{proof}
\hspace{-6mm}%Plugging in the condition  $kt>m$ to the lemma 9, we conclude if there exists an active column, with probability at least $1-\epsilon$ it will be detected within $\log{\frac{1}{\epsilon}}$ phases.
In the rest of the proof we show that with probability at least $1-e^{-T\frac{kt}{m}}$, estimated rank $\widehat{r}$ is equal to $r$.
$$P(r=\widehat{r}) = 1- \big( P(r<\widehat{r}) + P(r>\widehat{r})\big)$$
$P(r<\widehat{r}) = 0$ trivially satisfied, $\widehat{r}$ represents number of detected linearly independent columns of $\mathbf{M}$ which is always bounded by $r$.
Now, all we need to do is to bound $P(r<\widehat{r}) $.
We denote the event of existence of active column by $ACE$. Then, trivially: 
$$P(\widehat{r} < r) = P\big(\widehat{r} < r \hspace{1mm} \text{and} \hspace{1mm} ACE\big)$$
Moreover, we can write 
$$P\big(\widehat{r}< r \hspace{1mm} \text{and} \hspace{1mm} ACE\big) =\sum_{i=0}^{r-1} P\big(\widehat{r}= i \hspace{1mm} \text{and} \hspace{1mm} ACE\big)=
 P\big( ACE  \hspace{1mm} | \hspace{1mm} \widehat{r}= i \big) P(\widehat{r}=i) $$
To finish the proof we just need to observe following equality / inequality :
\begin{align*}
P(\widehat{r} < r) = \sum_{i=0}^{r-1} P\big(\widehat{r} = i  \wedge  ACE \big) 
= \sum_{i=0}^{r-1} P\big(ACE  |  \widehat{r} = i \big) P(\widehat{r}=i)
\end{align*}
From the lemma above, we can imply that  $$P\big(ACE  |  \widehat{r} = i \big) \leq e^{-T\frac{kt}{m}}$$ and as probability of $P(\widehat{r}=r)\neq 0$, we conclude $P(\widehat{r}<r) < 1$. Equivalently,
$$\sum_{i=0}^{r-1} P\big(\widehat{r}=i\big) < 1$$ which all together these two inequalities concludes 
\begin{align*}
P(\widehat{r} < r) =\sum_{i=0}^{r-1} P\big(ACE  |  \widehat{r} = i \big) P(\widehat{r}=i) \leq e^{-T\frac{kt}{m}}  \sum_{i=0}^{r-1} P(\widehat{r}=i) \leq e^{-T\frac{kt}{m}}
\end{align*}
To finalize the proof, we divide the algorithm $\mathbf{ERRE}$ into two parts.
First part, is the detection point of the last independent column by algorithm, and second part is waiting T many rounds to check if there is any independent column left.
Moreover, $\mathbf{ERRE}$ would fail generating correct matrix only if failure in the second part happens (there is still independent column not detected, but checking tells us that there is no left) i.e. $\widehat{r} < r$ which we just show $P(\widehat{r} < r) < e^{-T\frac{kt}{m}}$.
This concludes that with probability at least $1-e^{-T\frac{kt}{m}}$ recovered matrix is correct.\medskip \\
Therefore, with probability $1-e^{-T\frac{kt}{m}}$ the first part of the algorithm is just equivalent to the algorithm \hyperlink{err}{$\mathbf{ERR}$}, which with probability more than $1-\epsilon$
observation complexity is bounded by 
\begin{align*}
  (m+n-r)r +  \mathrm{min} \Big(  2 \frac{m n}{k}\log{(\frac{4r}{\epsilon})} , \frac{\frac{2m}{k}(r+2 +\log{\frac{1}{\epsilon}})}{t}n  \Big)     
\end{align*}
using the union bound we conclude that with probability at least $1-\epsilon+e^{-T\frac{kt}{m}}$, the algorithm recovers underlying matrix correctly and observation complexity is bounded by
\begin{align*}
  (m+n-r)r + Tn + \mathrm{min} \Big(  2 \frac{m n}{k}\log{(\frac{4r}{\epsilon})} , \frac{\frac{2m}{k}(r+2 +\log{\frac{1}{\epsilon}})}{t}n  \Big)     
\end{align*}
\end{proof}
\begin{corollary*} \label{cor:erre}Lets assume that either $\psi(\mathbb{U})$ or $\psi(\mathbb{V})$ is big enough i.e. $\psi(\mathbb{U})\psi(\mathbb{V}) \geq m$. {For} a given $\epsilon$ lets  set $T=\log{\frac{1}{\epsilon}}$, then $\mathbf{ERRE}$ recovers underlying matrix with probability $1-2\epsilon$  using just 
\begin{align*}
  (m+n-r)r+ n\log{\frac{1}{\epsilon}} +  \mathrm{min} \Big(  2 \frac{m n}{\psi(\mathbb{U})}\log{(\frac{r}{\epsilon})} , \frac{\frac{2m}{\psi(\mathbb{U})}(r+2 +\log{\frac{1}{\epsilon}})}{\psi(\mathbb{V})}n  \Big)     
\end{align*}
\end{corollary*}
\begin{proof}
We first observe following inequality as implication of given conditions:
\begin{align*} 
    kt \geq m  \implies   \frac{kt}{m} \geq 1 \implies e^{\frac{kt}{m}}\geq e \implies  e^{-\frac{kt}{m}}\leq \frac{1}{e}
\end{align*}
The rest of the proof is just straightforward application of the theorem. 
Setting $T = \log{\frac{1}{\epsilon}}$ to the statement of theorem tells with probability at least $1- ( \epsilon + e^{-\frac{kt}{m} \log{\frac{1}{\epsilon}}})$ using 
\begin{align*}
  (m+n-r)r+ n\log{\frac{1}{\epsilon}} +  \mathrm{min} \Big(  2 \frac{m n}{k}\log{(\frac{4r}{\epsilon})} , \frac{\frac{2m}{k}(r+2 +\log{\frac{1}{\epsilon}})}{t}n  \Big)     
\end{align*}
observations.
Considering the fact that $e^{-\frac{kt}{m}}\leq \frac{1}{e}$ we conclude  that 
\begin{align*}
 e^{-\frac{kt}{m} \log{\frac{1}{\epsilon}}}\leq  
\Big( \frac{1}{e} \Big)^{\log{\frac{1}{\epsilon}}} 
= e^{-\log{\frac{1}{\epsilon}}} = e^{\log{\epsilon}} = \epsilon
\end{align*}
Which concludes that with probability at least $1-2\epsilon$ the observation complexity is  bounded by 
\begin{align*}
  (m+n-r)r+ n\log{\frac{1}{\epsilon}} + \mathrm{ min} \Big(  2 \frac{m n}{k}\log{(\frac{4r}{\epsilon})} , \frac{\frac{2m}{k}(r+2 +\log{\frac{1}{\epsilon}})}{t}n  \Big)     
\end{align*}
\end{proof}
%\todo{tell that it is valuable for other k,t as as well. and if kt is small then space is coherent. which is the case algorithm fails. Discussing how big is nlog(1/epsilon) is also useful using previous corollary}

\newpage

\section{Proof of Theorem \ref{thm:erei}.  Exact Recovery with Two Phases}

Lets remind that in the algorithm \hyperlink{erei}{$\mathbf{EREI}$} we define
$\mathrm{min} \Big(  2 \frac{m }{\psi(\mathbb{U})}\log{(\frac{r}{\epsilon})} , \frac{\frac{2m}{\psi(\mathbb{U})}(r+2 +\log{\frac{1}{\epsilon}})}{\psi(\mathbb{V})}  \Big)$.
Basically there is two case to show algorithm recovers the underlying matrix correctly with probability $1-\epsilon$.

\subsection{ $d =  2 \frac{m }{\psi(\mathbb{U})}\log{(\frac{r}{\epsilon})} $}

We first start with the case that if minimum of these two quantities is $2 \frac{m }{k}\log{(\frac{r}{\epsilon})}$.
As the matrix has rank $r$, there exists at least one set of linearly independent columns with $r$ columns.
We select the set of linear independent columns$-C$ that has lexicographically smallest indices. 
We show sampling  $2 \frac{m }{k}\log{(\frac{1}{\epsilon})}$ entries from each column will give us the probability of at least $1-r\epsilon$ correctly recovery.\medskip\\
From the \hyperlink{step5}{Step 5} of proof of the theorem \ref{thm:erre} we can see sampling $2 \frac{m }{k}\log{(\frac{1}{\epsilon})}$ entries from an active column, would give guarantee of probability of at least $1-\epsilon$ detection of independence.
As $C$ is lexicographically smallest, each column is active on the time entries sampled from it, and each of $r$ columns will succeed with probability at least $1-\epsilon$.
Therefore, using union bound,  with probability $1-r\epsilon$ all of the columns in C will succeed, which guarantees the exact recovery. \medskip\\
Replacing $\epsilon$ by $\frac{\epsilon}{r}$ will conclude the result that sampling $2 \frac{m }{k}\log{(\frac{r}{\epsilon})}$  from each column will guarantees the correctness of the algorithm with probability at least $1-\epsilon$.

\subsection{ $d = \frac{\frac{2m}{\psi(\mathbb{U})}(r+2 +\log{\frac{1}{\epsilon}})}{\psi(\mathbb{V})}  $ }

From the follow up of lemma \ref{lemma:prob_bound}, we conclude that in a process of $\frac{k}{m}$ probability success and $1-\frac{k}{m}$ probability of failure, having 
$\frac{2m}{k}\big(r+2 +\log{\frac{1}{\epsilon}}\big)$ trial is enough to guarantee getting $r$ many success with at least probability $1-\epsilon$.\medskip\\
Failure probability of the algorithm $\mathbf{EREI}$ is equal to failing finding $r$ linearly independent columns. 
Consider following equation:
\begin{align*}
    P\big(\mathbf{EREI} fails \big) &= P\Big(\mathbf{EREI} fails \text{ and TNAO}  \geq \frac{2m}{k}\big(r+2 +\log{\frac{1}{\epsilon}}\big)\Big) \\
    &+P\Big(\mathbf{EREI} fails \text{ and TNAO}  < \frac{2m}{k}\big(r+2 +\log{\frac{1}{\epsilon}}\big)\Big) 
\end{align*}
where we denote TNAO as total number of active observations. 
Recall that we call an observation active, if it is active in the execution time (the column is still not contained in the current column space).
Intuitively we represent NAO by number of active observations executed by the algorithm $\mathbf{EREI}$ in the given specific time.\medskip\\
From lemma \ref{lem:activecolumns}, if there exists an active column, then there exists at least $t$ many active columns.
Therefore, failure of the algorithm is equivalent to existence of an active column when algorithm terminates.
Moreover each of our observations in those columns were active observations and considering the fact that we observed  $ \frac{\frac{2m}{k}\big(r+2 +\log{\frac{1}{\epsilon}}\big)}{t}$ many entries in each of them, total number of active observations is at least 
\begin{align*}
t \frac{\frac{2m}{k}\big(r+2 +\log{\frac{1}{\epsilon}}\big)}{t} =    
\frac{2m}{k}\Big(r+2 +\log{\frac{1}{\epsilon}}\Big)
\end{align*}
Therefore 
$P\Big(\text{NAO}  < \frac{2m}{k}\big(r+2 +\log{\frac{1}{\epsilon}}\big) | \mathbf{EREI} fails \Big) = 0$ and using Bayesian rule we conclude 
\begin{align*}
P\Big(\mathbf{EREI} fails \text{ and TNAO}  \leq \frac{2m}{k}\big(r+2 +\log{\frac{1}{\epsilon}}\big)\Big)=0    
\end{align*}
Then, following equation simplly satisfied:
\begin{align*}
    P\big(\mathbf{EREI} fails \big) = P\Big(\mathbf{EREI} fails \text{ and TNAO}  \geq \frac{2m}{k}\big(r+2 +\log{\frac{1}{\epsilon}}\big)\Big) 
\end{align*}
We can observe the following inequality as $\mathbf{EREI}$  may tamporarily fail at the point that the number of active observations is $\frac{2m}{k}\big(r+2 +\log{\frac{1}{\epsilon}}\big)$ but it can succeed finding remaining independent columns later during the execution:
\begin{align*}
    P\Big(\mathbf{EREI} \text{ currently fail when NAO =}&\frac{2m}{k}\big(r+2 +\log{\frac{1}{\epsilon}}\big) \Big) \geq\\
    &P\Big(\mathbf{EREI} fails \text{ and TNAO}  \geq \frac{2m}{k}\big(r+2 +\log{\frac{1}{\epsilon}}\big)\Big) 
\end{align*}
Therefore we conclude that:
\begin{align*}
    P\big(\mathbf{EREI} fails \big) \leq 
        P\Big(\mathbf{EREI} \text{ currently fail when NAO =}&\frac{2m}{k}\big(r+2 +\log{\frac{1}{\epsilon}}\big) \Big)
\end{align*}
Remember the fact that at each active observation probability of $\mathbf{EREI}$ detecting linear independence of  is larger or equal than $\frac{k}{m}$. 
From the previous discussion if the probability is exactly equal to $\frac{k}{m}$ then still not finding $r$ linearly independent column at $\frac{2m}{k}\big(r+2 +\log{\frac{1}{\epsilon}}\big)$ observations is less than $\epsilon$.
Therefore, $\mathbf{EREI}$ not detecting r linearly independent column after $\frac{2m}{k}\big(r+2 +\log{\frac{1}{\epsilon}}\big)$ observations is smaller than $\epsilon$, which is equivalent to 
\begin{align*}
    P\big(\mathbf{EREI} fails \big) \leq  \epsilon
\end{align*} 
as desired.\\\\
%\todo{make clear what is NAO and active columns and observations. Fix the algrotihm to the correct version ;) in the text}

\newpage

\section{Sparse Random Noise} 

We first start with the discussion regarding the \textit{sparsity-number} of row space of induced matrix:
\begin{lemma}
Lets assume that for a given $m\times n$ sized rank$-r$ matrix $\widetilde{\mathbf{M}}$, the \textit{nonsparsity-number} of it row space $\widetilde{\mathbb{V}}$ is equal to one: $\psi(\widetilde{\mathbb{V}})=1$. 
Then there is a column$-c$, that deletion of it decrements the rank: $\mathrm{rank}(\widetilde{\mathbf{M}}_{:[n]\setminus \{c\}})= r-1$.
\end{lemma}
\begin{proof}
From the definition of \textit{nonsparsity-number}, we notice that, it is always positive and moreover, only case that it is equal to $1$ is if some of the standard basis vector $e_i$ is contained in the space.
Then lets assume that the row space contains $e_{i_0}$, then we claim that the deletion of the column $i_0$ decrements the rank.\medskip\\
Lets assume that $\mathrm{rank}(\widetilde{\mathbf{M}}_{:[n]\setminus \{i_0\}})= r$.
Moreover, lets denote the $\widetilde{\mathbf{M}}^0$ by the matrix that is $i_0$-th column replaced by zero vector.
It is trivial to see that that 
$\mathrm{rank}(\widetilde{\mathbf{M}}_{:[n]\setminus \{i_0\}})= \mathrm{rank}(\widetilde{\mathbf{M}}^0)$.
Therefore $\mathrm{rank}(\widetilde{\mathbf{M}}^0) = r$ satisfies.
Moreover, row space of $\widetilde{\mathbf{M}}^0$ is subset of row space of $\widetilde{\mathbf{M}}$, however, as both of them has the same rank $r$, these space are the same.
But, this is a contradiction to the fact that, $e_{i_0}$ is contained in the row space of $\widetilde{\mathbf{M}}$ but not in the row space of $\widetilde{\mathbf{M}}^0$ (due to the fact that, entire row space has $0$ in its $i_0$-th coordinate).
Then, our assumption is wrong, $\mathrm{rank}(\widetilde{\mathbf{M}}_{:[n]\setminus \{i_0\}})$ cannot be $r$ and only other possible option is $r-1$.
Therefore $\mathrm{rank}(\widetilde{\mathbf{M}}_{:[n]\setminus \{c\}})= r-1$ satisfies.
\end{proof}
\begin{lemma}
Lets assume that for a given $m\times n$ sized rank$-r$ matrix $\widetilde{\mathbf{M}}$ with row space $\widetilde{\mathbb{V}}$, several columns are deleted. 
Then, rank of the matrix is preserved, and its non-sparsity number is decreased by at most $a-$where $a$ stands for the number of columns those are deleted.
\end{lemma}
\begin{proof}
The proof is just inductively application of following claims:
\vspace{-2mm}
\begin{itemize}
    \item[1] Deletion of single column, can reduce \textit{nonsparsity-number} by at most 1.
\vspace{-2mm}
    \item[2] if $\psi(\widetilde{\mathbb{V}}) > 1$, deletion of a column cannot decrement the rank.
\end{itemize} 
Lets prove the first claim:
Lets assume for contradiction that, there is a column $c$ that its deletion causes drop of row space
\textit{nonsparsity-number} by 2, i.e. $\psi(\widetilde{\mathbb{V}}) - \psi(\mathbb{V}') \geq 2$, 
where $\mathbb{V}'$ is the row space of $\widetilde{\mathbf{M}}_{:[n]\setminus \{c\} }$.
Let remind that the definition of \textit{nonsparsity-number}:
$\psi(\mathbb{V}')=\mathrm{min}\{\psi(x) | x\in \mathbb{V}' \text{ and } x\neq 0 \}$.
Lets pick the nonzero vector $x_0 \in \mathbb{V}'$ which satisfies the minimality in this definition.
As $\mathbb{V}'$ is restriction of $\widetilde{\mathbb{V}}$ to the index set $[n]\setminus \{c\}$, there is a vector $y \in \mathbb{V}$ such that $y_{[n]\setminus \{c\} } = x_0$. Therefore $\|y\|_0 \leq \|x_0\|_0 + 1 =  \psi(\mathbb{V}')+1$. 
Considering, $\psi(\widetilde{\mathbb{V}}) \leq \|y\|_0 \leq \|x_0\|_0 + 1 =  \psi(\mathbb{V}')+1$
which implies $\psi(\widetilde{\mathbb{V}}) -  \psi(\mathbb{V}') \leq 1$ and this contradicts to the assumption. 
Therefore, first claim indeed always satisfied. \medskip\\
Now, we prove the second claim:
This is a simple statement, once we notice that if deletion of the column $c$ results decrement in the rank of the matrix, then $e_c$ (i.e. $c-$th standard vector) is contained in the row space of $\widetilde{\mathbf{M}}$. The proof is simple as following:\\
Lets assume without lost of generality columns with the index set $\mathcal{B}=\{c_1,c_2,\ldots,c_{r-1},c\}$ is a basis for column space.
Note that, $c$ should be part of any basis, because without column$-c$ the column space has dimension $r-1$. 
Moreover, we know that for any $i\notin \mathcal{B}$, the column $\widetilde{\mathbf{M}}_{:i}$ can be written as linear combination of columns $\{c_1,c_2,\ldots,c_{r-1}\}$ i.e. $\widetilde{\mathbf{M}}_{:i}= \sum_{j=1}^{r-1}\alpha_j \widetilde{\mathbf{M}}_{:c_j}$ for scalar $\alpha_j$'s.
Moreover, considering the fact that, $\widetilde{\mathbf{M}}_{:\mathcal{B}}$ has rank equal to $r$, we can find the set of rows $R=\{R_1,R_2,\ldots, R_r\}$, that $\mathbf{M}_{R:\mathcal{B}}$ also has rank $r$. 
Considering the fact that, $\widetilde{\mathbf{M}}_{R:\mathcal{B}}$ is $r\times r$ sized matrix, then its row space contains the standard basis vector: $(0,0,\ldots,0,1)$.
This follows that there is a linear combination of rows $R=\{ R_1,R_2,\ldots,R_r \}$ with some scalars $\beta_1,\beta_2,\ldots, \beta_r$ that 
\begin{align*}
\beta_1 \widetilde{\mathbf{M}}_{R_1:\mathcal{B}} + \beta_2 \widetilde{\mathbf{M}}_{R_2:\mathcal{B}} + \ldots + \beta_r \widetilde{\mathbf{M}}_{R_r:\mathcal{B}} = (0,0,\ldots,0,1).    
\end{align*}
For a given $i\notin \mathcal{B}$ lets check the $i-$th coordinate of the vector
\begin{align*}
\beta_1 \widetilde{\mathbf{M}}_{R_1:i} + \beta_2 \widetilde{\mathbf{M}}_{R_2:i} + \ldots + \beta_r \widetilde{\mathbf{M}}_{R_r:i}.
\end{align*}
Remember that $\widetilde{\mathbf{M}}_{:i}= \sum_{j=1}^{r-1}\alpha_j \widetilde{\mathbf{M}}_{:c_j}$ as $i\notin \mathcal{B}$, therefore the sum above can be written as:
\begin{align*}
\beta_1 \widetilde{\mathbf{M}}_{R_1:i} + \beta_2 \widetilde{\mathbf{M}}_{R_2:i} + \ldots + \beta_r \widetilde{\mathbf{M}}_{R_r:i} &= 
\beta_1  \sum_{j=1}^{r-1}\alpha_j \widetilde{\mathbf{M}}_{:c_j} +
\beta_2  \sum_{j=1}^{r-1}\alpha_j \widetilde{\mathbf{M}}_{:c_j} + \ldots +
\beta_r  \sum_{j=1}^{r-1}\alpha_j \widetilde{\mathbf{M}}_{:c_j} \\
&= \alpha_1 \sum_{i=1}^{r} \beta_i \widetilde{\mathbf{M}}_{:c_1} +
\alpha_2 \sum_{i=1}^{r} \beta_i \widetilde{\mathbf{M}}_{:c_2} + \ldots +
\alpha_{r-1} \sum_{i=1}^{r} \beta_i \widetilde{\mathbf{M}}_{:c_{r-1}}  \\
&= \alpha_1 \times 0 + \alpha_2 \times 0 + \ldots + \alpha_{r-1}\times  0 = 0
\end{align*}
and this concludes that
\begin{align*}
\beta_1 \widetilde{\mathbf{M}}_{R_1:} + \beta_2 \widetilde{\mathbf{M}}_{R_2:} + \ldots + \beta_r \widetilde{\mathbf{M}}_{R_r:} = (0,0,\ldots,0,1,0,\ldots,0)
\end{align*}
Therefore $e_c$ is in the row space, and this implies that $\psi(\widetilde{\mathbb{V}}) = 1$.     Therefore,if $\psi(\widetilde{\mathbb{V}}) > 1$ then deletion of a column cannot decrement rank.
\end{proof}
\begin{algorithm}
\caption*{  \hypertarget{eerei}{\textbf{EEREI:}} Extended Exact recovery with estimated information}
\textbf{Input:}   $r, \psi(\mathbb{U}), \psi(\mathbb{V})$\\
 \textbf{Initialize:}  $k=0 , \widehat{\mathbf{U}}^0 = \emptyset, d = 2 \frac{m }{\psi(\mathbb{U})}\log{(\frac{r}{\epsilon})} , R=\emptyset$  
 
\begin{algorithmic}[1]
    \STATE if $\xi \leq \frac{\psi(\mathbb{V})}{2}$
    \STATE \hspace{0.2in} $d =  \mathrm{min}\Big(  2 \frac{m }{\psi(\mathbb{U})}\log{(\frac{r}{\epsilon})} , \frac{\frac{4m}{\psi(\mathbb{U})}(r+2 +\log{\frac{1}{\epsilon}})}{\psi(\mathbb{V})} \Big) $

    \STATE Draw uniformly random entries $\Omega \subset [m]$ of size $d$   
    \FOR{$i$ from $1$ to $n$}        
    \STATE  \hspace{0.2in} \textbf{if} $\| \mathbf{M}_{\Omega:i}-{\mathcal{P}_\mathbf{\widehat{U}_{\Omega}^k}} \mathbf{M}_{\Omega:i}\| >0$ 
    \STATE \hspace{0.2in}  \hspace{0.2in} Fully observe $\mathbf{M}_{:i}$ 
    \STATE  \hspace{0.2in}  \hspace{0.2in}  $\widehat{\mathbf{U}}^{k+1} \leftarrow \widehat{\mathbf{U}}^{k} \cup \mathbf{M_{:i}} $, Orthogonalize  $\widehat{\mathbf{U}}^{k+1}$, $k=k+1$          
    \STATE  \hspace{0.2in}  \hspace{0.2in}  Select a row $a \in \Omega \setminus R$ that, $\mathbf{\widehat{U}_{  R\cup \{a\}}^{k+1}}$ is rank $k+1$ then
    $R \leftarrow R \cup \{a\}$
    \STATE \hspace{0.2in} Draw uniformly random entries $\Delta \subset [m]\setminus R$ of size $d$ and $\Omega = \Delta \cup R$   
\ENDFOR
    \STATE Observe unobserved entries in $\mathbf{M}_{R:}$ 
    \FOR{$i$ from $1$ to $n$}        
       \STATE   \hspace{0.2in}  \textbf{if $\mathbf{M}_{:i}$} \text{ not fully observed : } $\widehat{\mathbf{M}}_{:i} = \widehat{\mathbf{U}}^k {\widehat{\mathbf{U}}^{k^+}_{R:}}
 \widehat{\mathbf{M}}_{R :i}$
 \ENDFOR
 \STATE  Detect all the columns that their deletion decrements rank and collect them in $\Sigma$
\end{algorithmic}
%\algorithmicindent \textbf{Output:} return $\widehat{\mathbf{M}}$
\textbf{Output:}  Noisy Columns - $\Sigma$, recovered underlying matrix $\widehat{\mathbf{M}}_{:[n]\setminus \Sigma}$
\end{algorithm}
The proof of the algorithm $\mathbf{EEREI}$ correctly detects noisy columns is the same as the proof provided in \cite{nina}, therefore we don't see necessity to provide it here.
Moreover, the correct recovery of the remaining entries is the same as the proof of $\mathbf{EREI}$
with only difference, if $\xi \leq \frac{\psi(\mathbb{V})}{2}$ happens and  $2 \frac{m }{\psi(\mathbb{U})}\log{(\frac{r}{\epsilon})} > \frac{\frac{4m}{\psi(\mathbb{U})}(r+2 +\log{\frac{1}{\epsilon}})}{\psi(\mathbb{V})} $.
However, the crucial step here will be to notice number of active columns will be at least $\frac{\psi(\mathbb{V})}{2}$ and at each active column we are doing $\frac{\frac{4m}{\psi(\mathbb{U})}(r+2 +\log{\frac{1}{\epsilon}})}{\psi(\mathbb{V})}$ many observations which gives overall
\begin{align*}
\frac{\frac{4m}{\psi(\mathbb{U})}(r+2 +\log{\frac{1}{\epsilon}})}{\psi(\mathbb{V})} \times  \frac{\psi(\mathbb{V})}{2}= 2 \frac{m}{\psi(\mathbb{U})}(r+2+\log{\frac{1}{\epsilon}})    
\end{align*}
active observations, which is the required number of active observations in order to detect $r$ complete column space with probability $1-\epsilon$.

\paragraph{Number of Observations:}
The number of observations is simply $\xi$ many additional observed columns and rows, compared to the algorithm $\mathbf{EREI}$ with the slight difference
if  $\xi < \frac{\psi(\mathbb{V})}{2}$ then
\begin{align*}
(m+n-r)r +  \mathrm{min}\Big(  2 \frac{m n}{\psi(\mathbb{U})}\log{(\frac{r}{\epsilon})} , \frac{\frac{4m}{\psi(\mathbb{U})}(r+2 +\log{\frac{1}{\epsilon}})}{\psi(\mathbb{V})}n \Big)  +\xi(m+n)
\end{align*}
and if $\xi > \frac{\psi(\mathbb{V})}{2}$
\begin{align*}
(m+n-r)r +  2 \frac{m n}{\psi(\mathbb{U})}\log{(\frac{r}{\epsilon})} +\xi(m+n)
\end{align*}

\subsection{Recall for properties of non-degenerate subspace}

Lets remind the characteristics of non-degenerate random vectors provided in \cite{nina}:\medskip\\
Let $\mathbf{E}^s \in \mathbb{R}^{m\times s}$ be matrix consisting of corrupted vectors drawn from any non-degenerate distribution. Let $\mathbb{U}^k ∈ \mathbb{R}^{m\times k}$ be any fixed matrix with rank $k$. Then with probability 1, we have
\begin{itemize}
    \item $\mathrm{rank}(\mathbf{E}^s)= s$ for any $s \leq m$
    \item $\mathrm{rank}(\mathbf{E}^s,x)= s+1$ holds for $x\in \mathbf{U}^k\subset \mathbb{R^m}$ uniformly and $s \leq m-k$, where $x$ can be depend or independent on $\mathbf{E}^s$
    \item $\mathrm{rank}(\mathbf{E}^s,\mathbb{U}^k)= s+k$ given that $s+k\leq m$ 
    \item The marginal of non-degenerate distribution is non-degenerate 
\end{itemize}
 
\newpage

\section{Bounded Deterministic Noise}

Proofs here are inspired by the work of \cite{nina}, with the given difference that here we use different$-$ smaller observation complexity.
For sake of completeness of the proof, we prove all details here as well.\medskip\\
We first show that, estimated subspace by algorithm does not have higher dimension than $r$. 
Then we provide upper bound to the error of recovered matrix.

\begin{lemma}
Let assume that $\mathbf{M}$ is can be decomposed as rank $r$ matrix $\mathbf{L}$ with additional small noise in each column that, its $\ell_2$ norm is bounded by $\epsilon$.
Then, at the end of the termination of the algorithm $\hyperlink{lrebn}{\mathbf{LREBN}}$, estimated subspace $\noisyksub$ has dimension at most $r$.
\end{lemma}
\begin{proof}
We prove that in the execution of the algorithm, we show if a column $\mathbf{M}_{:t}$ has been detected as new column that cannot be contained in pre-selected $\noisyksub$, then $\mathbf{L}_{:t}$ is indeed cannot be contained in the $\mathbf{U}^k$.
To use triangle inequality, we notice
\begin{align*}
\theta (\mathbf{L}_{:t},\mathbf{U}^k) \geq \theta (\mathbf{L}_{:t},\widetilde{\mathbf{U}}^k) - \theta (\widetilde{\mathbf{U}}^k, {\mathbf{U}}^k )    
\end{align*}
Using the lemma \ref{ks14} we can notice that following inequalities are get satisfied:
\begin{align*}
  \| \mathbf{M}_{\Omega t} - \mathcal{P}_{\noisyksub_{\Omega}} \mathbf{M}_{\Omega:t} \| &\leq 
\sqrt{\frac{3d}{2m}} \Big( \| \mathbf{M}_{:t} - \projnoisy \mathbf{M}_{:t} \| \Big) \\[1.3ex]
&\leq \sqrt{\frac{3d}{2m}} \Big( \| \mathbf{M}_{:t}-\mathbf{L}_{:t}\| +
 \|  \mathbf{L}_{:t} - \projnoisy  \mathbf{L}_{:t} \|  \Big) +
 \| \projnoisy ( \mathbf{L}_{:t}-\mathbf{M}_{:t} )\|   \\[1.3ex]
 &\leq \sqrt{\frac{3d}{2m}} \Big( \epsilon + \theta (\mathbf{L}_{:t},\widetilde{\mathbf{U}}^k)+\epsilon \Big)
\end{align*}
From the design of the algorithm  $ \| \mathbf{M}_{\Omega t} - \mathcal{P}_{\noisyksub_{\Omega}} \mathbf{M}_{\Omega:t} \|  > (1+\epsilon)\Big( \sqrt{\frac{3d}{2m}} \theta ({\mathbf{U}}^k, \noisyksub) +  \sqrt{\frac{3d k \epsilon}{2m}} \Big)$
and using this inequality above, we conclude that
\begin{align*}
\sqrt{\frac{3d}{2m}} \theta ({\mathbf{U}}^k, \noisyksub) +  \sqrt{\frac{3d k \epsilon}{2m}}    <   \sqrt{\frac{3d}{2m}} \Big( \epsilon + \theta (\mathbf{L}_{:t},\widetilde{\mathbf{U}}^k)+\epsilon \Big)
\end{align*}
which follows that
\begin{align*}
 \theta ({\mathbf{U}}^k, \noisyksub) +  \sqrt{ k \epsilon }    <   \Big( \epsilon + \theta (\mathbf{L}_{:t},\widetilde{\mathbf{U}}^k)+\epsilon \Big)
\end{align*}
considering the fact that $\epsilon < \frac{1}{4 }$ we conclude that 
\begin{align*}
\theta (\mathbf{L}_{:t},\widetilde{\mathbf{U}}^k) \geq \theta (\mathbf{L}_{:t},\widetilde{\mathbf{U}}^k) + 2\epsilon - \sqrt{k \epsilon} > \theta ({\mathbf{U}}^k, \noisyksub) 
\end{align*}
therefore we conclude that  $\theta ({\mathbf{U}}^k, \noisyksub) < \theta (\mathbf{L}_{:t},\widetilde{\mathbf{U}}^k) $  and it follows that $\theta (\mathbf{L}_{:t},\mathbf{U}^k) > 0$. 
Moreover, one can see that after every time this inequality get satisfied, dimension of $\mathbf{U}^k$ increases by one, and considering the fact that $\mathbf{U}^k$'s are subspace of column space of $\mathbf{L}$, its dimension cannot increase more than $r$ times.
\end{proof}
Then only remaining step to provide an upper bound to recovery error.
Note that, if the algorithm decides completely observe the column, then $\ell_2$ norm of the error is upper bounded by $\epsilon$.
Then, all we need to do is to give upper bound to columns those recovered by estimated subspace.
\begin{align*}
\| \widetilde{\mathbf{M}}_{:t} -\mathbf{L}_{:t}  \| 
&= \| \noisyksub \noisyinverse_{\Omega:} \mathbf{M}_{\Omega t}- \mathbf{L}_{:t}\|  \\[1.3ex]
&\leq  \| \noisyksub \noisyinverse_{\Omega:} \mathbf{M}_{\Omega t}- \noisyksub \noisyinverse_{\Omega:} \mathbf{L}_{\Omega:t}  \| +
     \| \noisyksub \noisyinverse_{\Omega} \mathbf{L}_{\Omega:t} - \noisyksub \noisyinverse \mathbf{L}_{:t}\| +
\| \noisyksub \noisyinverse \mathbf{L}_{:t} -\mathbf{L}_{:t}\| \\[1.3ex]
&\leq  \| \noisyksub \noisyinverse_{\Omega:} ( \mathbf{M}_{\Omega t}- \mathbf{L}_{\Omega:t}) \| +
     \| \noisyksub \noisyinverse_{\Omega} \mathbf{L}_{\Omega:t} - \noisyksub \noisyinverse \mathbf{L}_{:t}\| + \sin{\theta(\mathbf{L}_{:t}, \widetilde{\mathbf{U}}^k)}  \\[1.3ex]
&\leq \| \noisyksub \noisyinverse_{\Omega:}\| \|(\mathbf{M}_{\Omega t}-\mathbf{L}_{\Omega:t}) \| +
\| \noisyksub \noisyinverse_{\Omega} \mathbf{L}_{\Omega:t} - \noisyksub \noisyinverse \mathbf{L}_{:t}\| +
\theta(\mathbf{L}_{:t}, \widetilde{\mathbf{U}}^k)
\end{align*}
Then all we need to do is to give an upper bound to the final term.
Lets start with the second term here: $\mathbf{L}_{:t} = \noisyksub v + e$ where $\noisyksub v = \noisyksub \noisyinverse \mathbf{L}_{:t}$ and note $\| e \| = \sin{\theta(\mathbf{L}_{:t}, \noisyksub)} \leq \theta(\mathbf{L}_{:t}, \noisyksub) $. Therefore:
\begin{align*}
\noisyksub \noisyinverse_{\Omega} \mathbf{L}_{\Omega:t} - \noisyksub \noisyinverse \mathbf{L}_{:t} = \noisyksub \noisyinverse_{\Omega} (\noisyksub v + e) - \noisyksub v = \noisyksub \noisyinverse_{\Omega} e
\end{align*}
Hence we conclude that:
\begin{align*}
\| \widetilde{\mathbf{M}}_{:t} -\mathbf{L}_{:t}  \| 
&\leq \| \noisyksub \noisyinverse_{\Omega:}\| \|(\mathbf{M}_{\Omega t}-\mathbf{L}_{\Omega:t}) \| +
\| \noisyksub \noisyinverse_{\Omega} e_{\Omega}\| +
\theta(\mathbf{L}_{:t}, \widetilde{\mathbf{U}}^k) \\[1.3ex]
&\leq \| \noisyksub \noisyinverse_{\Omega:}\| \|(\mathbf{M}_{\Omega t}-\mathbf{L}_{\Omega:t}) \| +
\| \noisyksub \noisyinverse_{\Omega}\|  \theta(\mathbf{L}_{:t}, \noisyksub) +
\theta(\mathbf{L}_{:t}, \widetilde{\mathbf{U}}^k). 
\end{align*}
To give upper bound to this expression, we notice  $ \| \noisyksub \noisyinverse_{\Omega:t} \| \leq \frac{ \sigma_1 (\widetilde{\mathbf{U}}^k)}{ \sigma_k(\widetilde{\mathbf{U}}^k_{\Omega:}) }\leq \Theta(\frac{m}{d})$ given the condition that $d\geq 4 \mu(\noisyksub) k \log{\frac{k}{\delta}} $ from the lemma \ref{matcher}.
From lemma \ref{noisycoh} we know that
$\mu(\noisyksub) \leq  2 \mu(\mathbf{U}^k) + 2 \frac{m}{k}\theta(\noisyksub,\mathbf{U}^k)^2$
and from lemma \ref{kcoh} we notice that $k \mu(\noisyksub) \leq r \mu(\mathbf{U})$. Then all together these facts concludes  the selected\\
$$d = 72 \mu(\mathbf{U}) r\log^2{\frac{1}{\delta}} + 8 m \theta(\noisyksub,\mathbf{U}^k)^2 \log{\frac{r}{\delta}} \geq 
8 \mu(\mathbf{U}) r\log{\frac{r}{\delta}} + 8 m \theta(\noisyksub,\mathbf{U}^k)^2 \log{\frac{r}{\delta}}$$ satisfies  $d\geq 4 \mu(\noisyksub) k \log{\frac{k}{\delta}} $ (it is assumed that $\delta \leq \frac{1}{r^{1/8}}$ ).
Therefore, we can bound $ \| \noisyksub \noisyinverse_{\Omega:t} \| $ above by 
$ \Theta(\frac{m}{d})$.\medskip\\
Now, only remaining term in the error bound above is $\theta(\mathbf{L}_{:t}, \noisyksub)$, and we use the following inequality to compare it with quantities provided as input:
\begin{align*}
    \| \projnoisy  \mathbf{M}_{:t} - \mathbf{L}_{:t}  \| \geq 
    \sin \theta( \projnoisy  \mathbf{M}_{:t} , \mathbf{L}_{:t}) \geq 
    \frac{\theta( \projnoisy  \mathbf{M}_{:t} , \mathbf{L}_{:t}) }{2} \geq
    \frac{ \theta( \noisyksub , \mathbf{L}_{:t}) }{2}
\end{align*}
and to relate the term  $ \| \projnoisy  \mathbf{M}_{:t} - \mathbf{L}_{:t}  \|$ with observed entries we again use the inequality \ref{ks14} and the fact that $\big(1+2\log{\frac{1}{\delta}} \big)^2 \leq 6 \log^2{\frac{1}{\delta}}$ once $\delta<0.1$, lemma \ref{kcoh} and lemma \ref{ededler}

\begin{align*}
    \|  \mathbf{M}_{\Omega:t}  -\projnoisy  \mathbf{M}_{\Omega:t}  \| &\geq
    \sqrt{ \frac{1}{m} \Big(\frac{d}{2} -\frac{3k \mu(\noisyksub)\beta}{2}  \Big) }  
     \|  \mathbf{M}_{:t}  -\projnoisy  \mathbf{M}_{:t}  \|    \\[1.3ex]
     &\geq \sqrt{ \frac{1}{m}\Big(\frac{d}{2} -\frac{3k \mu(\noisyksub)\beta}{2}  \Big) }  
\Big( \|\mathbf{L}_{:t}  -\projnoisy  \mathbf{M}_{\Omega:t}  \|-\| \mathbf{L}_{:t} - \mathbf{M}_{:t}\|  \Big) \\[1.3ex]
&\geq    \sqrt{ \frac{1}{m}\Big(\frac{d}{2} -\frac{3k \mu(\noisyksub)\beta}{2}  \Big) }  
\Big( \| \projnoisy  \mathbf{M}_{:t} - \mathbf{L}_{:t}  \| -\epsilon \Big) \\[1.3ex]
&\geq    \sqrt{ \frac{1}{m} \Big(\frac{d}{2} -\frac{3k \mu(\noisyksub)\beta}{2}  \Big) }  
\Big( \frac{\theta(\noisyksub, \mathbf{L}_{:t})}{2} -\epsilon \Big) \\[1.3ex]
&\geq   \sqrt{ \frac{1}{m} \Big(\frac{d}{2} -9k \mu(\noisyksub) \log^2{\frac{1}{\delta}}  \Big) }  
\Big( \frac{\theta(\noisyksub, \mathbf{L}_{:t})}{2} -\epsilon \Big) \\[1.3ex]
&\geq   \sqrt{ \frac{1}{m} \Big(\frac{d}{2} - 18 k\mu(\mathbf{U}^k) \log^2{\frac{1}{\delta}} -18m\theta(\noisyksub,\mathbf{U}^k)^2 \log^2{\frac{1}{\delta}} \Big) }
\Big( \frac{\theta(\noisyksub, \mathbf{L}_{:t})}{2} -\epsilon \Big) \\[1.3ex]
&\geq   \sqrt{ \frac{d}{2m} - \frac{18k}{m}\mu(\mathbf{U}^k) \log^2{\frac{1}{\delta}} -18\theta(\noisyksub,\mathbf{U}^k)^2 \log^2{\frac{1}{\delta}} } \Big( \frac{\theta(\noisyksub, \mathbf{L}_{:t})}{2} -\epsilon \Big) \\[1.3ex]
&\geq   \sqrt{ \frac{d}{2m} - \frac{18r}{m}\mu(\mathbf{U}) \log^2{\frac{1}{\delta}} -18\theta(\noisyksub,\mathbf{U}^k)^2 \log^2{\frac{1}{\delta}} } \Big( \frac{\theta(\noisyksub, \mathbf{L}_{:t})}{2} -\epsilon \Big) \\[1.3ex]
&\geq   \sqrt{\frac{d}{4m}} \Big( \frac{\theta(\noisyksub, \mathbf{L}_{:t})}{2} -\epsilon \Big)
\end{align*}
From here, we conclude that:
\begin{align*}
    \theta({\noisyksub, \mathbf{L}_{:t}})  \leq 4 \sqrt{\frac{m}{d}}   \|  \mathbf{M}_{\Omega:t}  -\projnoisy  \mathbf{M}_{\Omega:t}  \|  + 2 \epsilon  
    & \leq 4 \sqrt{\frac{m}{d}} (1+\epsilon)  \Big( \sqrt{\frac{3d}{2m}} \theta ({\mathbf{U}}^k, \noisyksub)  + \sqrt{\frac{3d k \epsilon}{2m}} + 2 \epsilon \Big)\\[1.ex]
    &\leq (1+\epsilon) \Big(\sqrt{24} \theta ({\mathbf{U}}^k, \noisyksub) +   \sqrt{8k \epsilon}  \Big)
\end{align*}
Finally, returning back to the recovery error: 
\begin{align*}
\| \widetilde{\mathbf{M}}_{:t} -\mathbf{L}_{:t}  \| 
&\leq \| \noisyksub \noisyinverse_{\Omega:}\| \|(\mathbf{M}_{\Omega t}-\mathbf{L}_{\Omega:t}) \| +
\| \noisyksub \noisyinverse_{\Omega}\|  \theta(\mathbf{L}_{:t}, \noisyksub) +
\theta(\mathbf{L}_{:t}, \widetilde{\mathbf{U}}^k)  \\[1.3ex]
&\leq \frac{m}{d} \epsilon +\Big( \frac{m}{d}+1\Big) \Big(\sqrt{24} \theta ({\mathbf{U}}^k, \noisyksub) +    \sqrt{8k \epsilon}   \Big)(1+\epsilon) 
\end{align*}
Then all we need to do is to give upper bound to $\theta(\noisyksub,\mathbf{U}^k)$. 
In the proof below, we use similar argument to \cite{blum}. 
Lets assume $\mathbf{U}^k = \{u_1,u_2,\ldots, u_k\}$ and 
$\noisyksub = \{\widetilde{u}_1,\widetilde{u}_2,\ldots, \widetilde{u}_k \}$ where each of $ \| u_i-\widetilde{u}_i \| \leq \epsilon$ satisfied. 
Then using triangle inequality, lemma \ref{blum} and lemma \ref{conc}
\begin{align*}
    \theta(\noisyksub,\mathbf{U}^k) &\leq \theta(\noisyksub, \widehat{\mathbf{U}}) + \theta(\widehat{\mathbf{U}}, \mathbf{U}^k) \\[1.5ex]
    &\leq \frac{\pi}{2} \frac{ \theta(u_k, \widetilde{u}_k) }{\theta(\widetilde{u}_k,\mathbf{U}^{k-1})} + \theta(\noisykcixbir, {\mathbf{U}}^{k-1} )\\[1.5ex]
    &\leq \frac{\pi}{2} \frac{ \theta(u_k, \widetilde{u}_k) }{\theta(\widetilde{u}_k,\noisykcixbir) -\theta(\noisykcixbir, {\mathbf{U}}^{k-1} ) } + \theta(\noisykcixbir, {\mathbf{U}}^{k-1} )  \\[1.5ex]
    &\leq \frac{\pi}{2} \frac{ \theta(u_k, \widetilde{u}_k) }{\sqrt{k \epsilon} + \theta(\noisykcixbir, {\mathbf{U}}^{k-1} ) -\theta(\noisykcixbir, {\mathbf{U}}^{k-1} ) } + \theta(\noisykcixbir, {\mathbf{U}}^{k-1} )   \\[1.5ex]
&\leq    \frac{\pi}{2} \frac{\epsilon}{\sqrt{k \epsilon}} + \theta(\noisykcixbir, {\mathbf{U}}^{k-1} ) 
\end{align*}
and using lemma \ref{ind}, we can conclude that $\theta(\noisyksub, {\mathbf{U}}^{k} ) \leq \frac{3\pi}{2} \sqrt{k \epsilon}$, which gives the final bound to 
$\| \widetilde{\mathbf{M}}_{:t} -\mathbf{L}_{:t}  \|$  to be $\Theta(\frac{m}{d}\sqrt{k\epsilon})$.

\begin{lemma} \label{conc}
Given that $\| \mathbf{M}_{\Omega t} - \mathcal{P}_{\noisykcixbir_{\Omega}}   \mathbf{M}_{\Omega:t} \| \geq (1+\epsilon)\Big( \sqrt{\frac{3d}{2m}} \theta(\noisykcixbir, \mathbf{U}^{k-1}) + \sqrt{\frac{3d k \epsilon}{2m}} \Big)$ satisfies. 
Then following also satisfies: 
\begin{align*}
    \theta(\widetilde{u}_k, \noisykcixbir) \geq  \theta(\noisykcixbir, \mathbf{U}^{k-1}) + \sqrt{k \epsilon}
\end{align*}
\end{lemma}
\begin{proof} Note that simple triangle inequality implies $\| \mathbf{M}_{:t}\| \leq 1+\epsilon$

\begin{align*}
 \theta(\widetilde{u}_k, \noisykcixbir) = \theta(\mathbf{M}_{:t}, \noisykcixbir) &\geq \sin \theta(\mathbf{M}_{:t}, \noisykcixbir)  \\[1.3ex]
 &\geq\frac{\mathbf{M}_{:t}}{1+\epsilon} \sin \theta(\mathbf{M}_{:t}, \noisykcixbir) \\[1.3ex]
 &= \frac{1}{1+\epsilon} \| \mathbf{M}_{:t} - \mathcal{P}_{\noisykcixbir} \mathbf{M}_{:t} \| \\[1.3ex]
 &\geq \frac{1}{1+\epsilon} \sqrt{\frac{2m}{3d}}  \| \mathbf{M}_{\Omega t} - \mathcal{P}_{\noisykcixbir_{\Omega}}   \mathbf{M}_{\Omega:t} \| 
\end{align*}\\
Using, the fact that 
$\| \mathbf{M}_{\Omega t} - \mathcal{P}_{\noisykcixbir_{\Omega}}   \mathbf{M}_{\Omega:t} \| \geq (1+\epsilon)\Big( \sqrt{\frac{3d}{2m}} \theta(\noisykcixbir, \mathbf{U}^{k-1}) + \sqrt{\frac{3d k \epsilon}{2m}} \Big)$ we conclude $\theta(\widetilde{u}_k, \noisykcixbir) \geq  \sqrt{k \epsilon} + \theta(\noisykcixbir, {\mathbf{U}}^{k-1} )$.
\end{proof}

\begin{lemma} \label{kcoh}
Let $\mathbf{U}^k$ be a $k$-dimensional subspace of $\mathbf{U}$ which is subspace of $\mathbb{R}^m$ with dimension $r$. Then following inequality satisfied:
\begin{align*}
    k\mu(\mathbf{U}^k) \leq r \mu(\mathbf{U})
\end{align*}
\end{lemma}
\begin{proof}
\begin{align*}
 k \mu(\mathbf{U}^k) = k \frac{m}{k}  \underset{1 \leq j \leq m}{\max} \|\mathcal{P}_{\mathbf{U}^k} e_i\|^2 &=
 r \frac{m}{r}  \underset{1 \leq j \leq m}{\max}  \|\mathcal{P}_{\mathbf{U}^k} e_i\|^2 \\
&\leq  r \frac{m}{r}   \underset{1 \leq j \leq m}{\max} \|\mathcal{P}_{\mathbf{U}} e_i\|^2 \\
 &= r\mu(\mathbf{U})   
\end{align*}
and the inequality due to $\mathbf{U}^k \subseteq \mathbf{U}$
\end{proof}

\begin{lemma} \label{ind}
Let assume that $a_0 = 0$ and $a_k \leq a_{k-1} + \frac{\pi}{2} \sqrt{\frac{\epsilon}{k}}$. Then it follows that $a_k \leq \frac{3\pi}{2} \sqrt{k\epsilon}$
\end{lemma}
\begin{proof}
Its trivial to notice that $a_{1}\leq \frac{\pi}{2} \sqrt{\epsilon} \leq 3\frac{\pi}{2} \sqrt{\epsilon} $.
Lets assume by induction for a given $k$ any index $i\leq k$ satisfies $a_i \leq 3\frac{\pi}{2}\sqrt{i\epsilon}$ and then we will prove that $a_{k+1} \leq 3 \frac{\pi}{2}\sqrt{(k+1)\epsilon}$.
We prove it by contradiction, by assuming $a_{k+1} > 3 \frac{\pi}{2}\sqrt{(k+1)\epsilon}$ and conclude to a contradiction.
\begin{align*}
    a_{k+1} &> 3 \frac{\pi}{2}\sqrt{(k+1)\epsilon} \\ 
     - a_k  &\geq -3 \frac{\pi}{2}\sqrt{k\epsilon}
\end{align*}
Therefore, $a_{k+1} - a_k \geq 3\frac{\pi}{2}\sqrt{\epsilon}\Big( \sqrt{k+1}-\sqrt{k} \Big) =
3\frac{\pi}{2}\sqrt{\epsilon} \frac{1}{\sqrt{k}+\sqrt{k+1}} \geq 3\frac{\pi}{2}\sqrt{\epsilon} \frac{1}{3 \sqrt{k}} = \frac{\pi}{2} \sqrt{\frac{\epsilon}{k}}$ which contradicts to the statement of the lemma.
Therefore, assumption cannot be satisfied which follows  $a_{k+1} \leq 3 \frac{\pi}{2}\sqrt{(k+1)\epsilon}$
\end{proof}

\begin{lemma} \label{noisycoh}
Let $\noisyksub$ and $\mathbf{U}^k$ be as defined above then, coherence number of these spaces satisfies the following inequality:
\begin{align*}
\mu(\noisyksub) \leq  2 \mu(\mathbf{U}^k) + 2 \frac{m}{k}\theta(\noisyksub,\mathbf{U}^k)^2
\end{align*}
\end{lemma}
\begin{proof}
In order to achieve the goal of comparing $\mu(\noisyksub)$ and $\mu(\mathbf{U}^k)$, we first need to understand how projection to standard vectors to $\mathbf{U}^k$ differ than projection of them to $\noisyksub$:
\begin{align*}
  \|    \projnoisy e_i \| \leq  \| \mathcal{P}_{\mathbf{U}^k} e_i \| +  \| \projnoisy e_i - \mathcal{P}_{\mathbf{U}^k} e_i \|  &\leq  \| \mathcal{P}_{\mathbf{U}^k} e_i \| +  \|  \projnoisy  - \mathcal{P}_{\mathbf{U}^k}   \|  \| e_i \| \\ 
  &=  \| \mathcal{P}_{\mathbf{U}^k} e_i \| +  \sin \theta(\noisyksub, \mathbf{U}^k) \\
  &\leq   \| \mathcal{P}_{\mathbf{U}^k} e_i \| +   \theta(\noisyksub, \mathbf{U}^k) 
\end{align*}
Therefore:
\begin{align*}
\mu(\noisyksub) = \frac{m}{k} \underset{1 \leq j \leq n}{\max} \| \projnoisy e_i \|^2 &\leq \frac{m}{k} \Big( 2 \underset{1 \leq j \leq n}{\max}  \| \mathcal{P}_{\mathbf{U}^k}e_i \|^2 + 2 \theta(\noisyksub,\mathbf{U}^k)^2 \Big) \\[1.3ex] 
&= 2 \mu(\mathbf{U}^k) + 2 \frac{m}{k}\theta(\noisyksub,\mathbf{U}^k)^2
\end{align*}
\end{proof}

\begin{lemma} \label{ededler}
Lets assume the setting as discussed in the proof above. 
Then,  
\begin{align*}
    \frac{d}{4m} > \frac{18r}{m}\mu(\mathbf{U}) \log^2{\frac{1}{\delta}} + 18\theta(\noisyksub,\mathbf{U}^k)^2 \log^2{\frac{1}{\delta}}
\end{align*}
\end{lemma}
\begin{proof}
Remind $d = 72 \mu(\mathbf{U}) r\log^2{\frac{1}{\delta}} + 8 m \theta(\noisyksub,\mathbf{U}^k)^2 \log{\frac{r}{\delta}} $ and it  implies
$\frac{d}{4m} = 18 \mu(\mathbf{U}) r\log^2{\frac{1}{\delta}} + 2 m \theta(\noisyksub,\mathbf{U}^k)^2 \log{\frac{r}{\delta}} $.
Then all we need to show is $2m \log{\frac{r}{\delta}} > 18 \log^2{\frac{1}{\delta}}$.
However, we always pick $\delta$ as $9 \log{\frac{1}{\delta}} < m$, simply because $m\geq d\geq 9\log{\frac{1}{\delta}}$  
\end{proof}

\begin{lemma} [\bf \cite{blum}] \label{blum}
Let subspaces $U$, $V$, and $\widetilde{V}$ defined as $U = span\{ a_1,\ldots, a_{k-1}\}$, $V = span\{ a_1,\ldots, a_{k-1},b\}$ and $\widetilde{V}= span\{ a_1,\ldots, a_{k-1}, \tilde{b}\}$. 
Then following inequality satisfied:
\begin{align*}
\theta( V, \widetilde{V}) \leq \frac{\pi}{2} \frac{\theta(\tilde{b},b)}{\theta(\tilde{b},U)}    
\end{align*}

\end{lemma}

\begin{lemma} [\bf \cite{akshay2}] \label{ks14}
Let $\noisyksub$ be a $k$-dimensional subspace of $\mathbb{R}^m$, and set 
$d = \mathrm{max} ( \frac{8}{3}k\mu(\noisyksub)\log{\frac{2k}{\delta}}, 4 \mu \mathcal{P}_{\noisyksub}  \log{\frac{1}{\delta}})$.
Given that $\Omega$ stands for uniformly selected subset of $[m]$ then following inequality get satisfied:
$$\frac{d(1-\alpha) -  k\mu(\noisyksub ) \frac{\beta}{1-\zeta} }{m}\|y-\projnoisy y \|  \leq \| y_{\Omega}- \mathcal{P}_{\noisyksub_{\Omega}}  y_{\Omega}\| \leq (1+\alpha) \frac{d}{m} \|y- \projnoisy y \|$$
where $\alpha =  \sqrt{ 2 \frac{ \mu(\mathcal{P}_{\widetilde{\mathbf{U}}^{k^\perp}} y)}{d} \log{\frac{1}{\delta}} } + 2\frac{\mu ( \mathcal{P}_{\widetilde{\mathbf{U}}^{k^\perp}} y)} {3d} \log{\frac{1}{\delta}}$  ,  $\beta=(1+2\log{1/\delta})^2$ and $\zeta = \sqrt{ \frac{8k \mu(\widetilde{\mathbf{U}}^{k^\perp})}{3d} \log{\frac{2r}{\delta}} }$
\end{lemma}
as noted in the paper, this lemma can be used by $\alpha < 1/2$ and $\gamma < 1/3$

\begin{lemma}  [\bf \cite{eigen}] \label{matcher}
Consider a finite sequence $\{ \mathbf{X}_k \} \in \mathbb{R}^{n\times n} $ independent random, Hermitian matrices those satisfies: 
\begin{align*}
    0 \leq \lambda_{\mathrm{min}}(\mathbf{X}_k) \leq \lambda_{\mathrm{max}}(\mathbf{X}_k) \leq  L.
\end{align*}
Let $\mathbf{Y} = \sum\limits_k \mathbf{X}_k$ and $\mu_r$ be the $r$-th largest eigenvalue of  $\mathbb{E}[\mathbf{Y}]$ ( $\mu_r =\lambda_r ( \mathbb{E}[\mathbf{Y}])$), then for any $\epsilon \in[0,1)$ following inequality  satisfied:
\begin{align*}
    \mathbf{Pr}( \lambda_r(\mathbf{Y}) \geq (1-\epsilon) \mu_r ) \geq 1-r \Big( \frac{e^{-\epsilon}}{(1-\epsilon)^{1-\epsilon}} \Big)^{\frac{\mu_r}{L}} \geq 1-r e^{\frac{\mu_r \epsilon^2 }{2L}} 
\end{align*}
\end{lemma}

\newpage

\section{Proofs for the design of Experiments}

\subsection{Design of coherent row and column space }

To design an $m\times n$ sized rank $r$ with \textit{space sparsity number} equal to $1$, we generate $m\times {r-1}$ and ${r-1}\times n$ sized matrices $\mathbf{X,Y}$, where $X_{i,j},Y_{i,j}\sim \mathcal{N}(0,1)$. 
As we discussed before, multiplication of these matrices would gives us a rank $r-1$ matrix.
Moreover, as the column space of $\mathbf{M}$ is column space of $\mathbf{Y}$.  Given that  $Y_{i,j} \sim \mathcal{N}(0,1)$ implies that coherence of column space of $\mathbf{Y}$ is small. Therefore, $\mathbf{M}$ has small column space coherence number.
We can use the similar argument to claim the coherence of column space is also small as row space of $\mathbf{M}$ is the row space of $\mathbf{X}$. \medskip\\
In order to make column space of this matrix highly coherent, we follow the following procedure:

\begin{itemize}
    \item[1.]   generate a random vector $u\in \mathbb{R}^n$
    \item[2.]   randomly select a number $i \in [m]$ 
    \item[3.]   replace  $\mathbf{M}_{i:}$ with $u$
\end{itemize}
We can guarantee that the resulting matrix will contain $i$-th standard basis vector $e_i$ in the column space. 
To observe this phenomenon, lets analyse the restriction of the matrix $\mathbf{M}$ to the first $r$ columns and all the rows but row $i$.
As this is a submatrix of rank $r-1$ matrix (initial $\mathbf{M}$) this matrix also has rank at most $r-1$.
Therefore, we have non-trivial coefficients $\alpha_1, \alpha_2, \ldots, \alpha_r$, that makes linear combination of columns of submatrix to be equal to zero vector.
Therefore,
\begin{align*}
\alpha_1 \mathbf{M}_{:1}+\alpha_1 \mathbf{M}_{:2}+\ldots+ \alpha_r\mathbf{M}_{:r} = w e_i
\end{align*}
for some $w$. Then all we need to show is $w \neq 0$, however it is straightforward because $w = \alpha_1 u_1+\alpha_2 u_2 +\ldots + \alpha_r u_r$ which is nonzero because $u$ is random. 
In conclusion, $e_i$ is contained in the column space of $\mathbf{M}$ and therefore from the definition of coherence of the columns space of the matrix is equal to $\frac{m}{r}$ which is also maximum value.\medskip\\
We note that, we might change the process above and generate several random vectors and replace them with some rows of the matrix, we would still get high coherence values as $\Omega(\frac{m}{r})$.
Using similar idea we can add replace columns with random vector to get highly coherent row spaced matrices.
Moreover, we can apply both at the same time, to get highly coherent column and highly coherent row space.

%\bibliography{reference}
%\bibliographystyle{plain}

%\end{document}
